# Supplementary material for: Diffusion Sampling with Momentum for Mitigating Divergence Artifacts
Source: arXiv:2307.11118 source file (2023-07-20)
Supplement: Supplementary file 1 [file ver1.tex]

\tabulinesep=1pt
\begin{figure}[ht]
    \centering
    \subcaptionbox{PLMS4 \cite{liu2022pseudo}}{
        \includegraphics[width=0.2\textwidth]{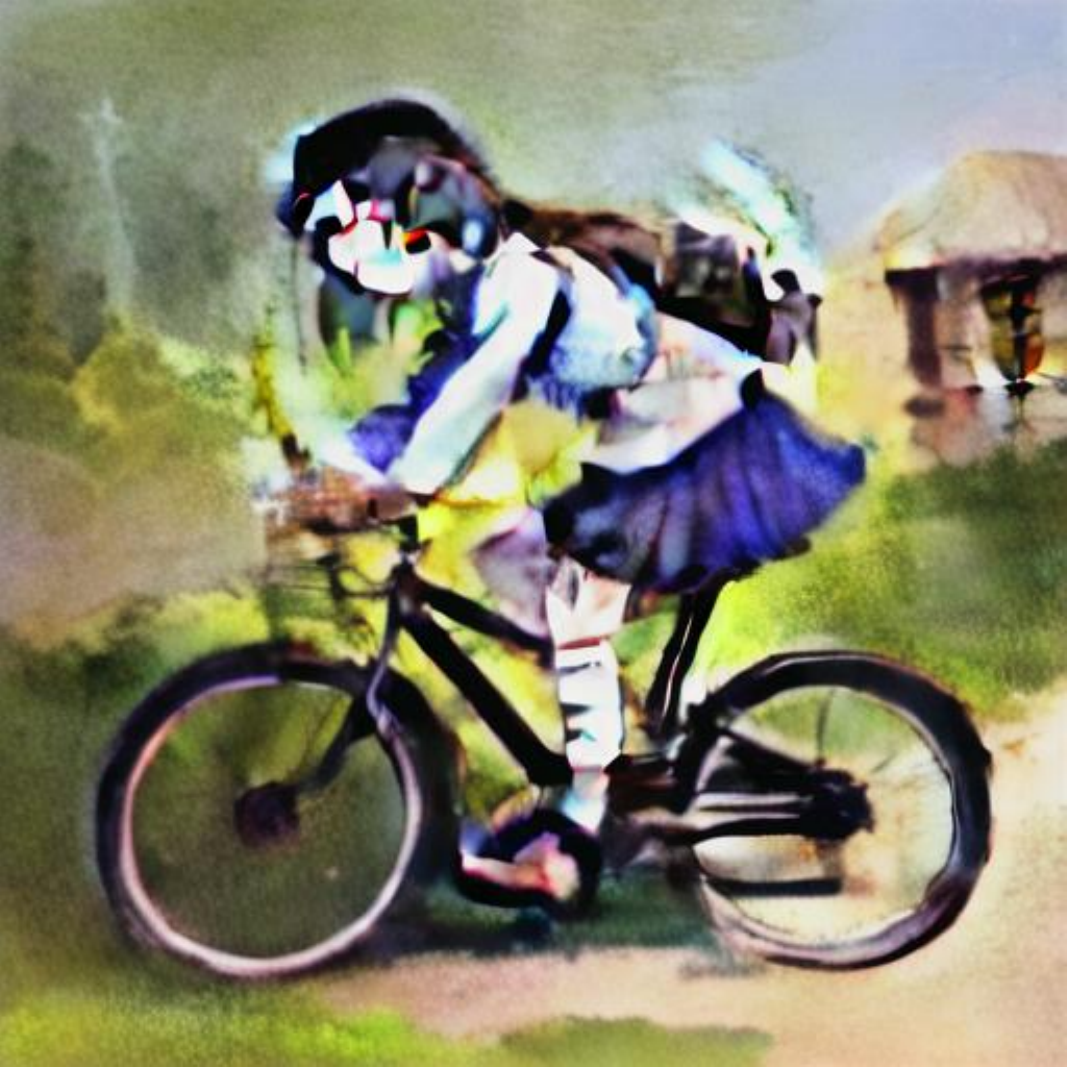}
        \hfill
        \includegraphics[width=0.2\textwidth]{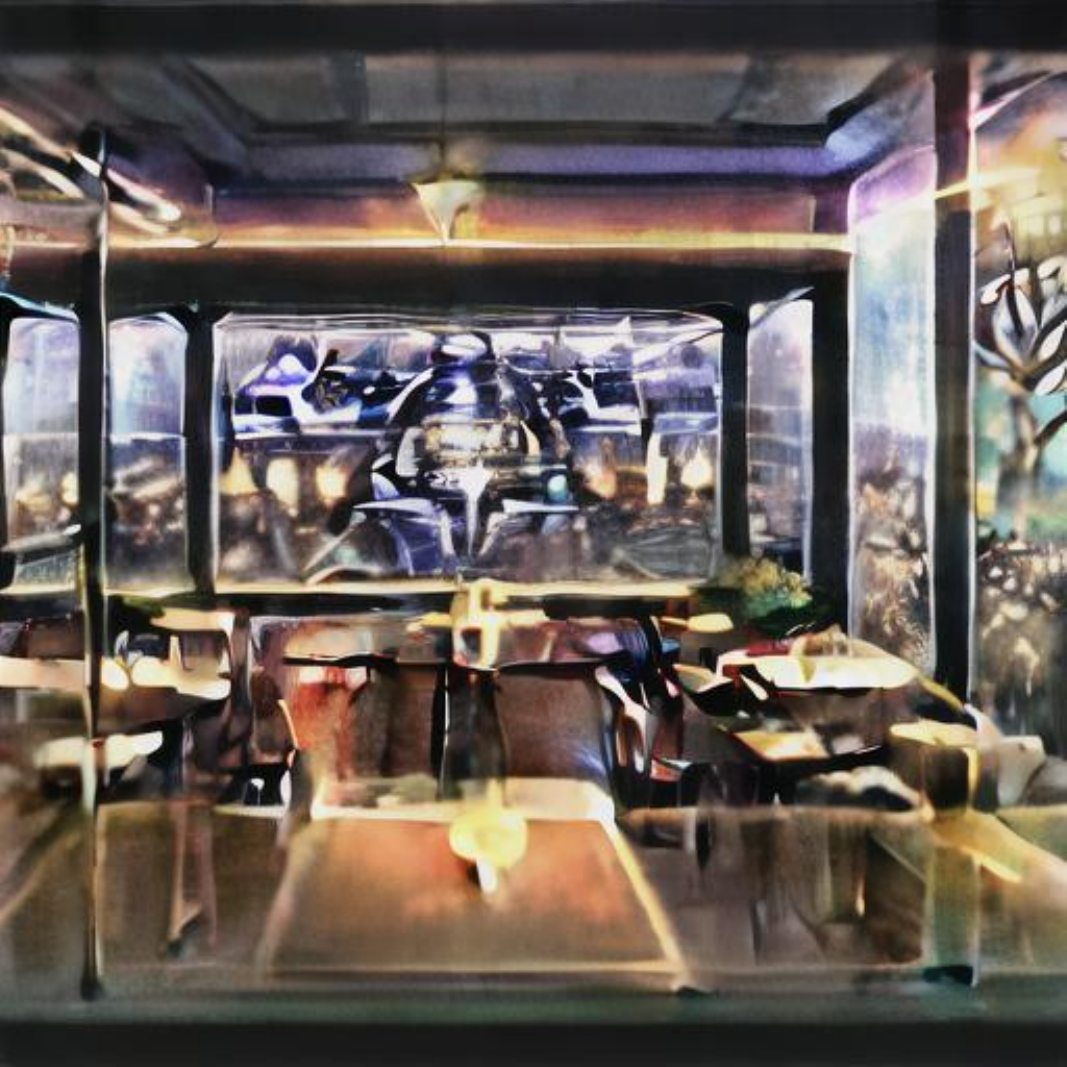}
        \hfill
        \includegraphics[width=0.2\textwidth]{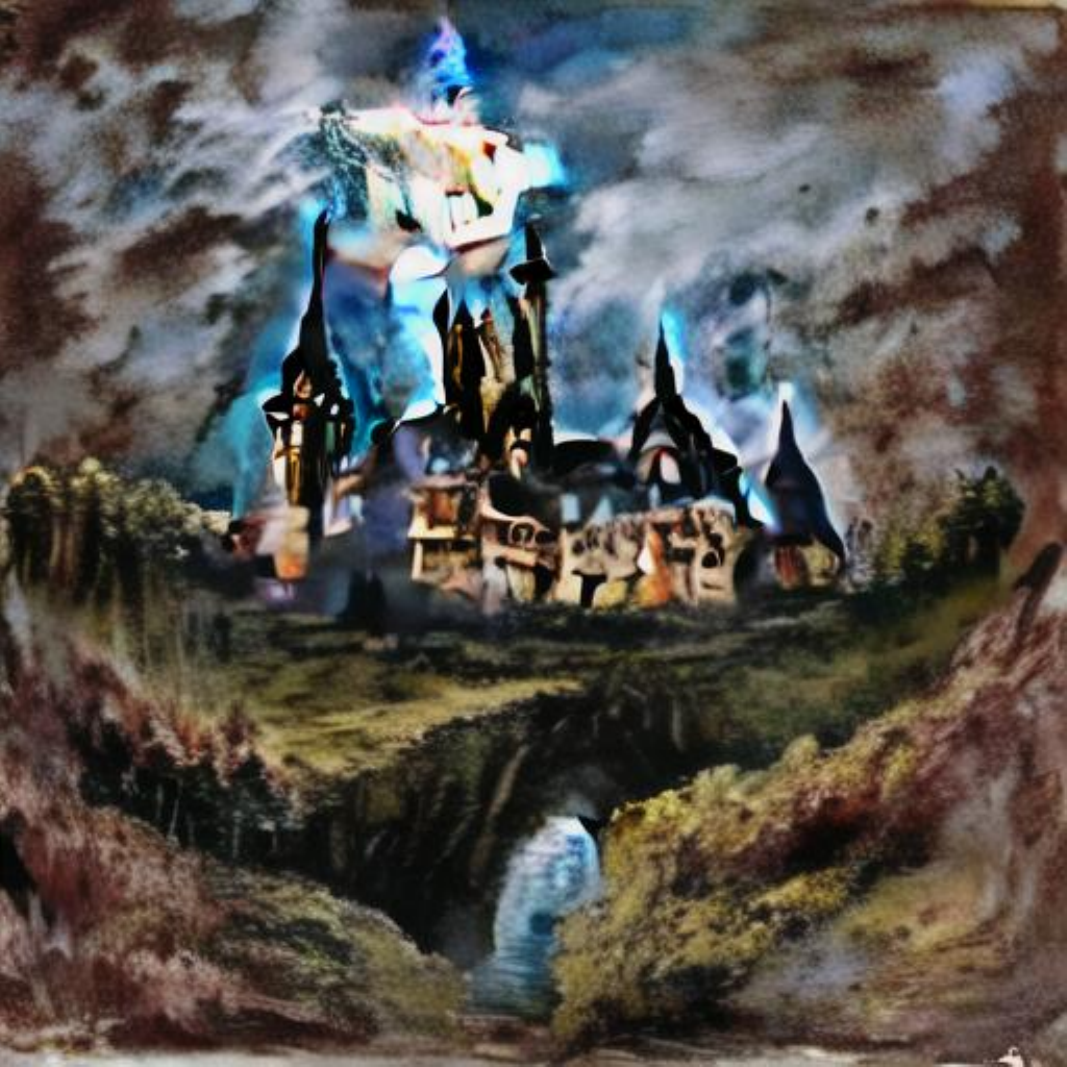}
    }
    \subcaptionbox{Prompt 1: bla bla bla}{
        \begin{tabu} to \textwidth {
            @{}
            l@{\hspace{6pt}}
            c@{\hspace{2pt}}
            c@{\hspace{2pt}}
            c@{\hspace{2pt}}
            c@{\hspace{2pt}}
            c@{}
        }
            % & \noindent\parbox[c]{0.17\columnwidth}{{DPM++ \cite{}}} 
            % & \multicolumn{4}{c}{\shortstack{\scriptsize DDIM \cite{} \\ \scriptsize 1000 steps}}
            & \multicolumn{1}{c}{\shortstack{\scriptsize $\beta = 0.2$}}
            & \multicolumn{1}{c}{\shortstack{\scriptsize $\beta = 0.4$}}
            & \multicolumn{1}{c}{\shortstack{\scriptsize $\beta = 0.6$}}
            & \multicolumn{1}{c}{\shortstack{\scriptsize $\beta = 0.8$}}
            & \multicolumn{1}{c}{\shortstack{\scriptsize $\beta = 0.9$}} \\
    
            \shortstack[l]{\scriptsize (a) w/ HB} &
            \noindent\parbox[c]{0.17\columnwidth}{\includegraphics[width=0.17\columnwidth]{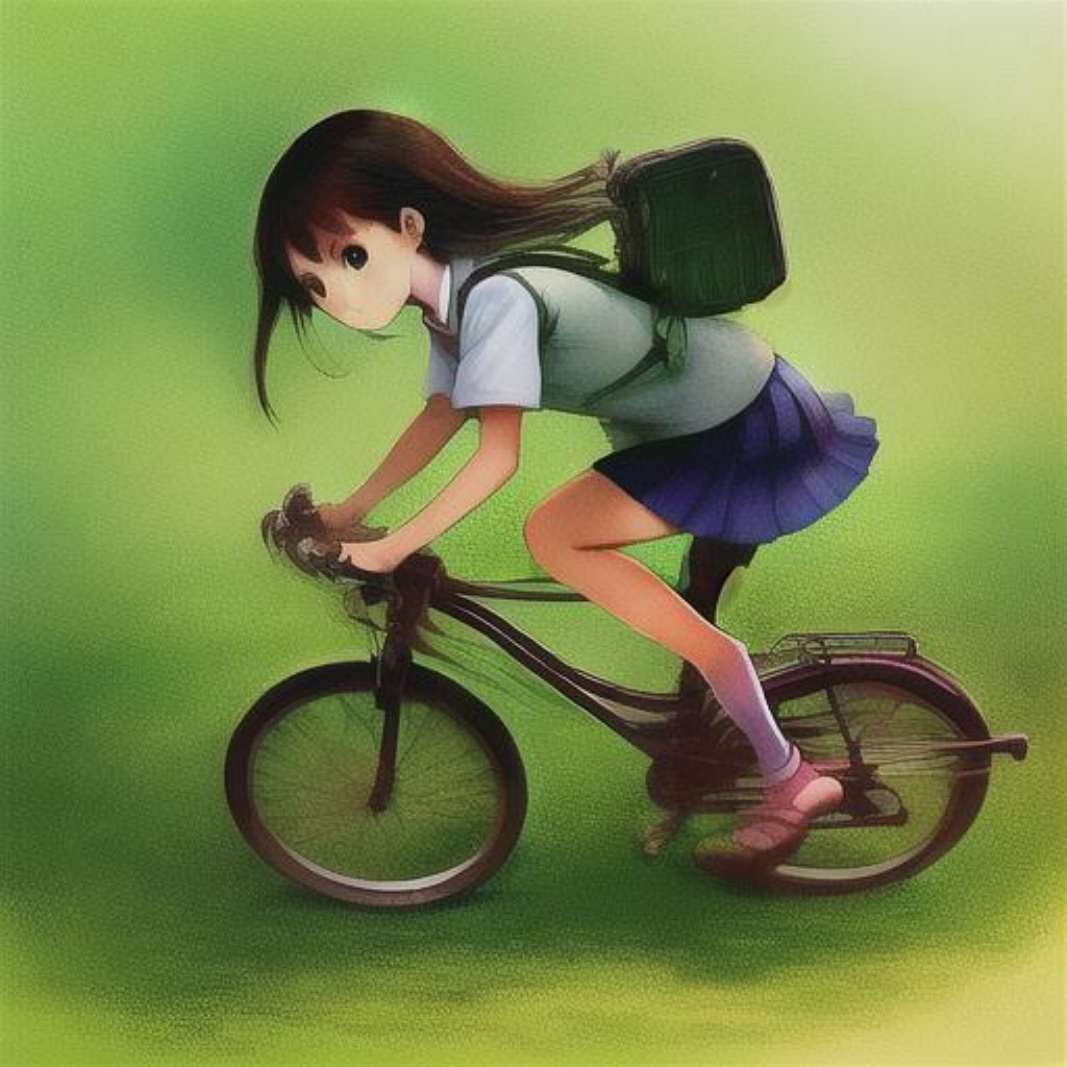}} & 
            \noindent\parbox[c]{0.17\columnwidth}{\includegraphics[width=0.17\columnwidth]{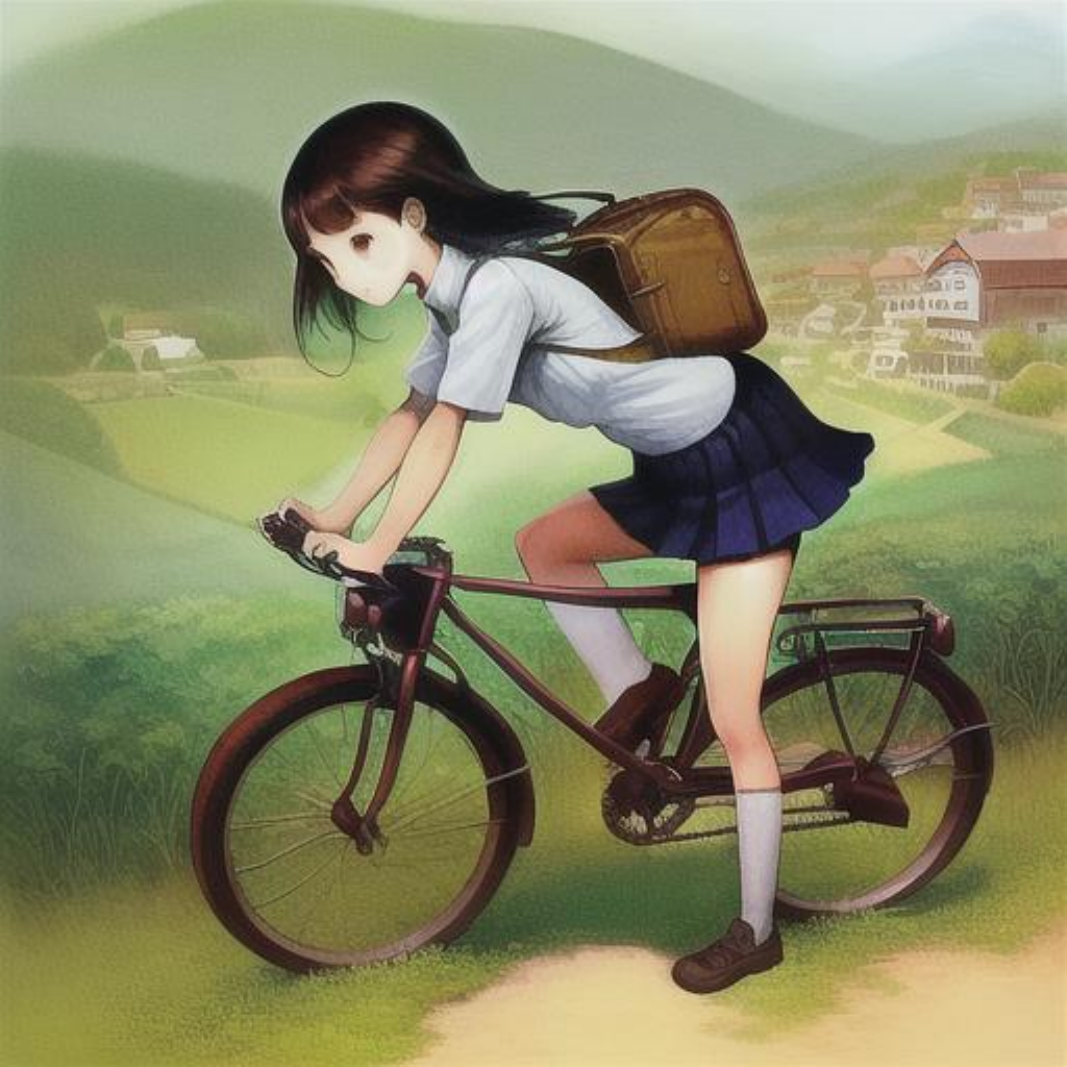}} & 
            \noindent\parbox[c]{0.17\columnwidth}{\includegraphics[width=0.17\columnwidth]{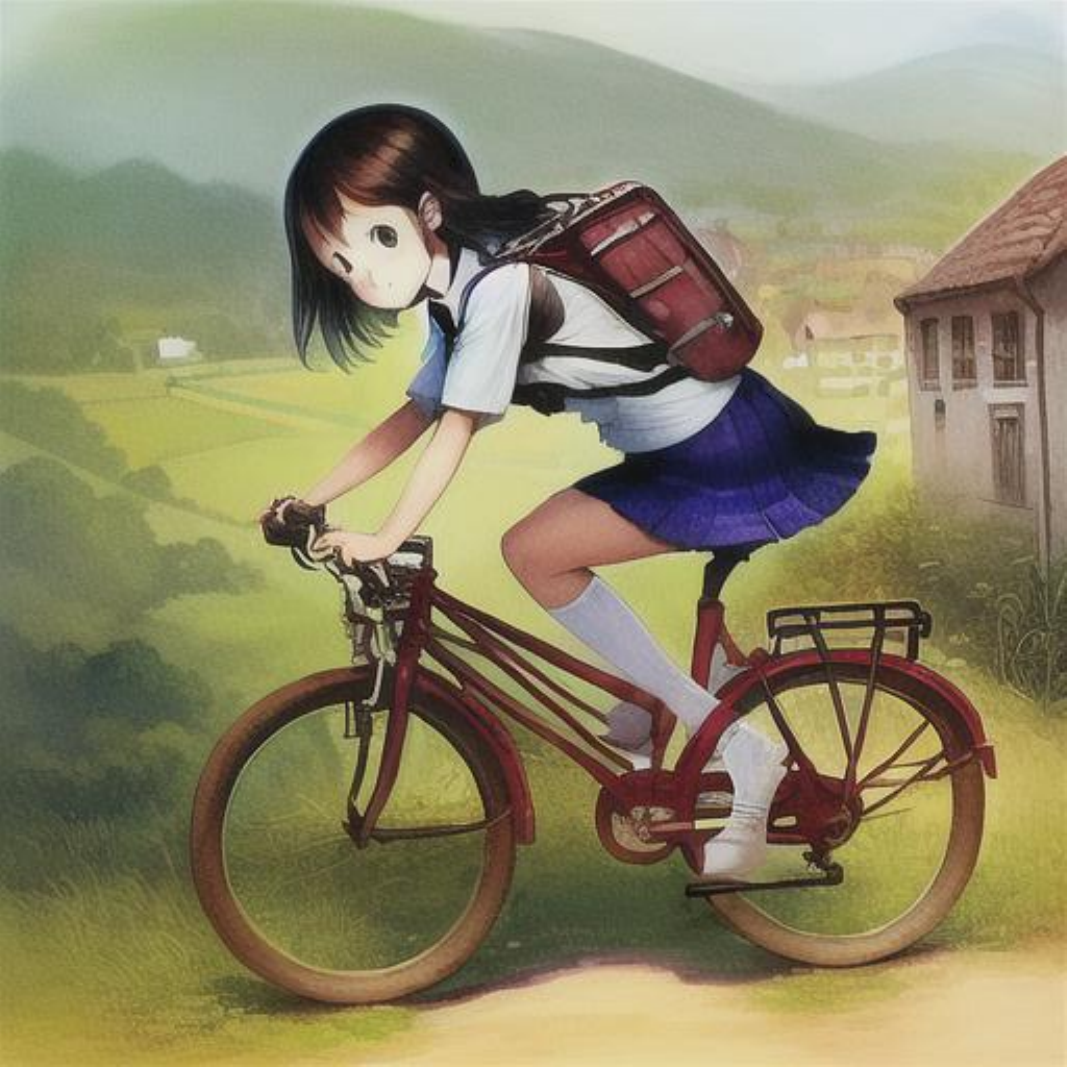}} & 
            \noindent\parbox[c]{0.17\columnwidth}{\includegraphics[width=0.17\columnwidth]{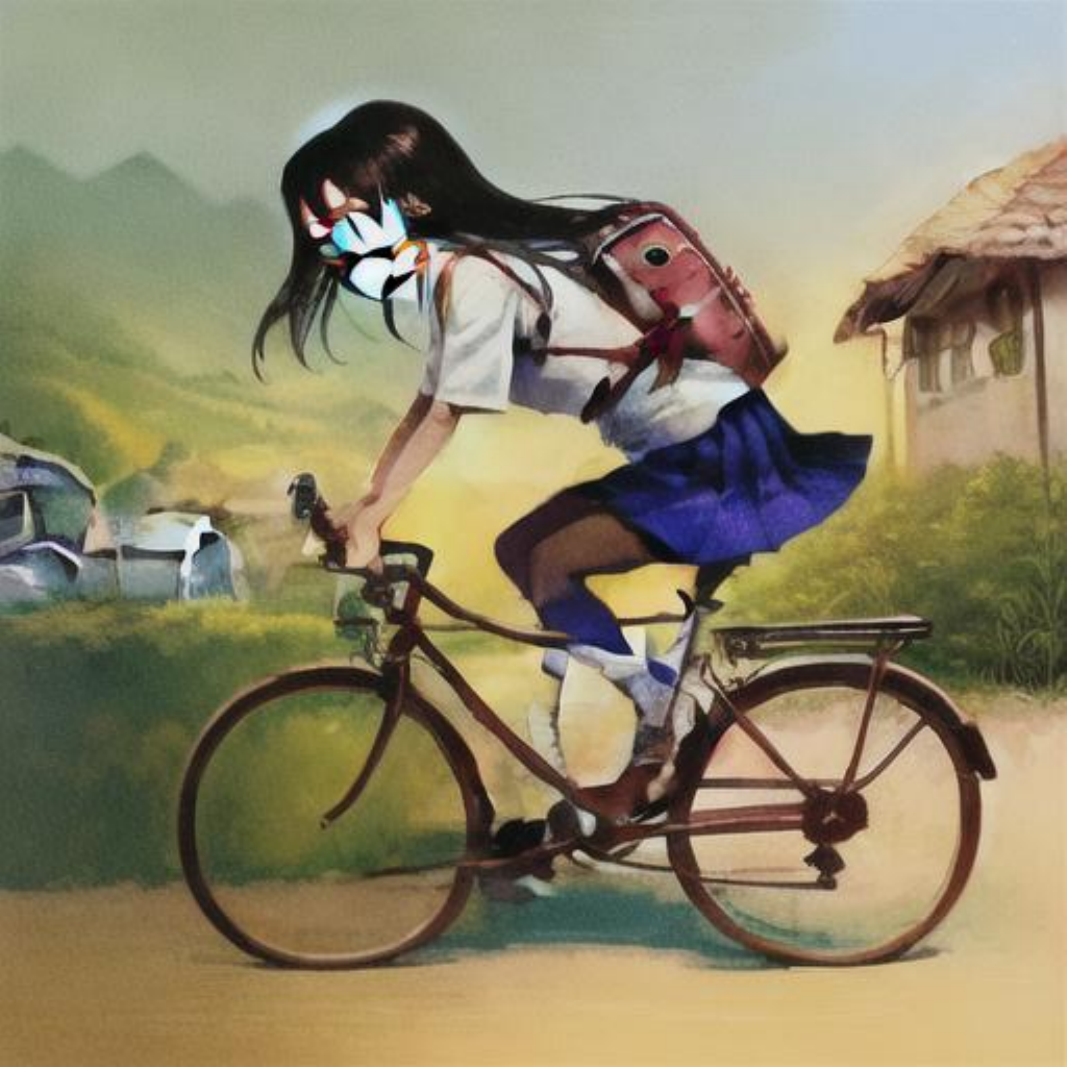}} & 
            \noindent\parbox[c]{0.17\columnwidth}{\includegraphics[width=0.17\columnwidth]{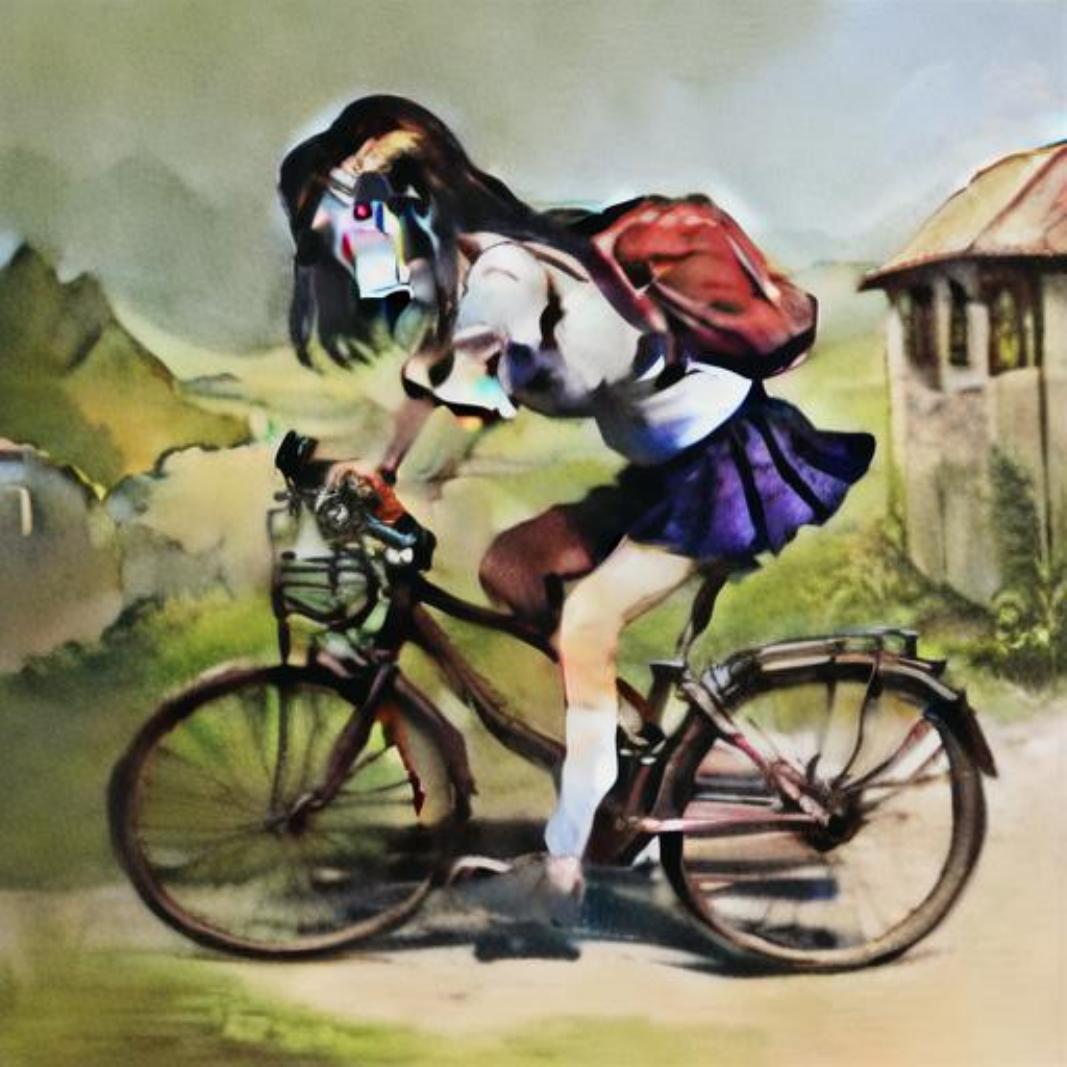}} \\
    
            & \multicolumn{1}{c}{\shortstack{\scriptsize $\beta = 0.2$}}
            & \multicolumn{1}{c}{\shortstack{\scriptsize $\beta = 0.4$}}
            & \multicolumn{1}{c}{\shortstack{\scriptsize $\beta = 0.6$}}
            & \multicolumn{1}{c}{\shortstack{\scriptsize $\beta = 0.8$}}
            & \multicolumn{1}{c}{\shortstack{\scriptsize $\beta = 0.9$}} \\
    
            \shortstack[l]{\scriptsize (a) w/ NT} &
            \noindent\parbox[c]{0.17\columnwidth}{\includegraphics[width=0.17\columnwidth]{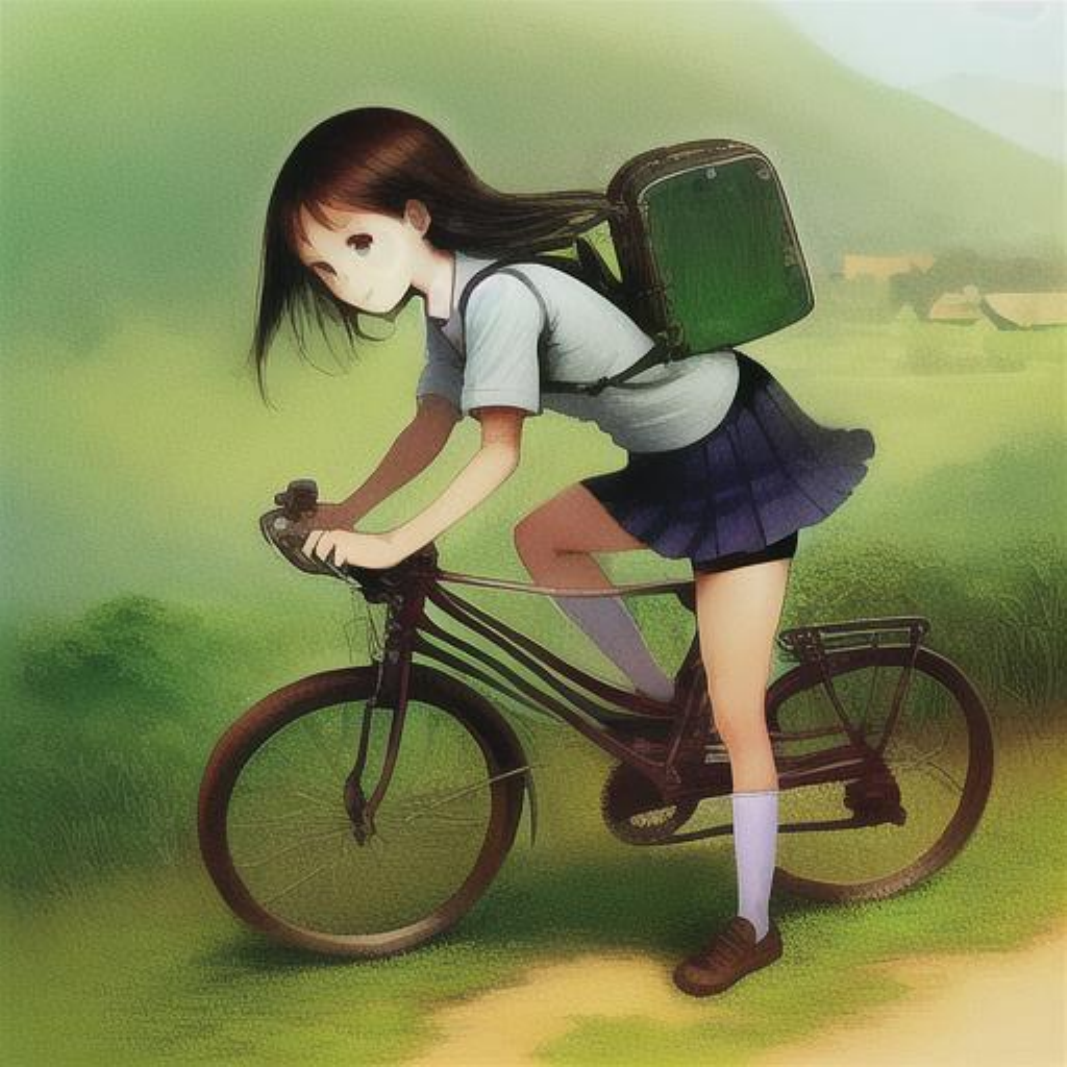}} & 
            \noindent\parbox[c]{0.17\columnwidth}{\includegraphics[width=0.17\columnwidth]{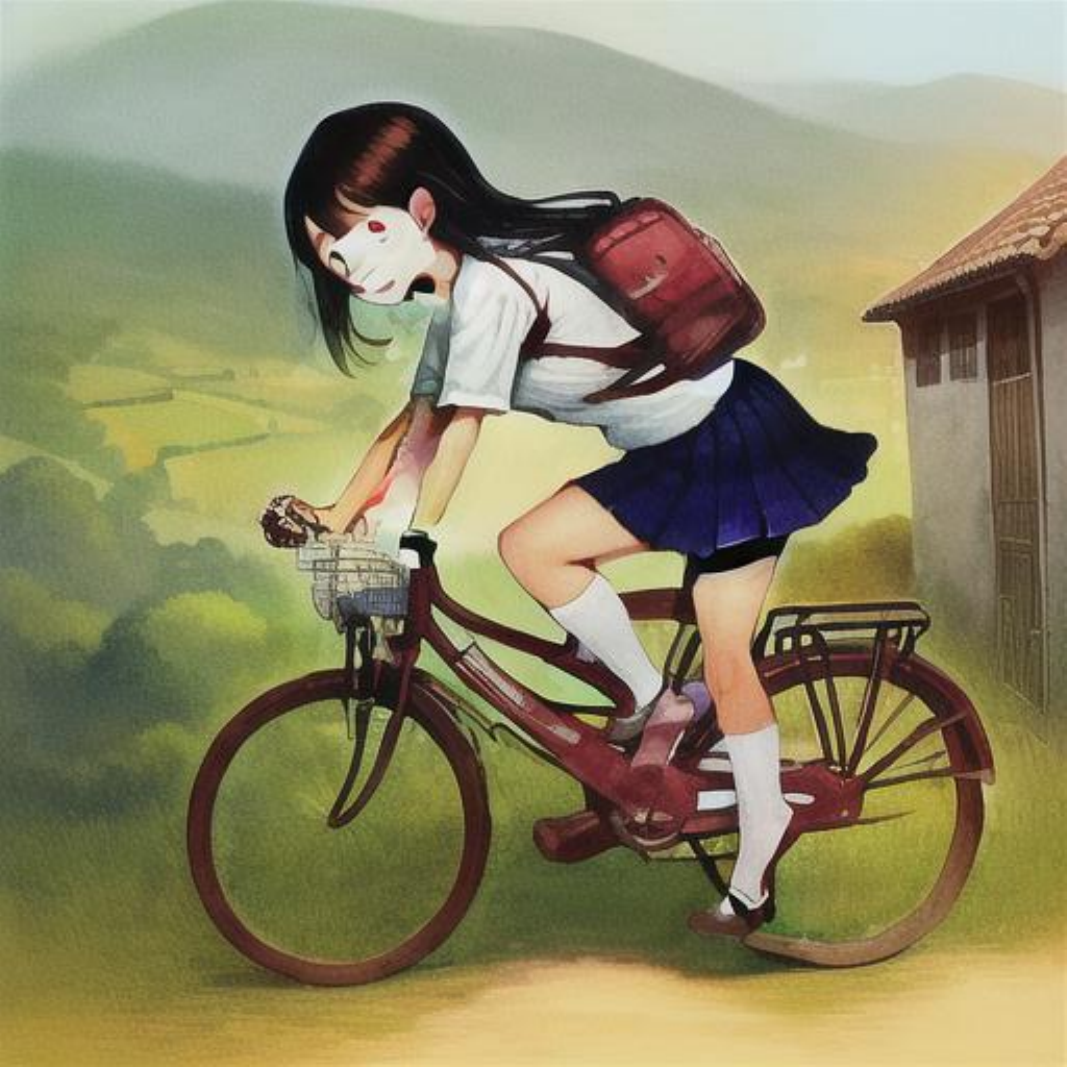}} & 
            \noindent\parbox[c]{0.17\columnwidth}{\includegraphics[width=0.17\columnwidth]{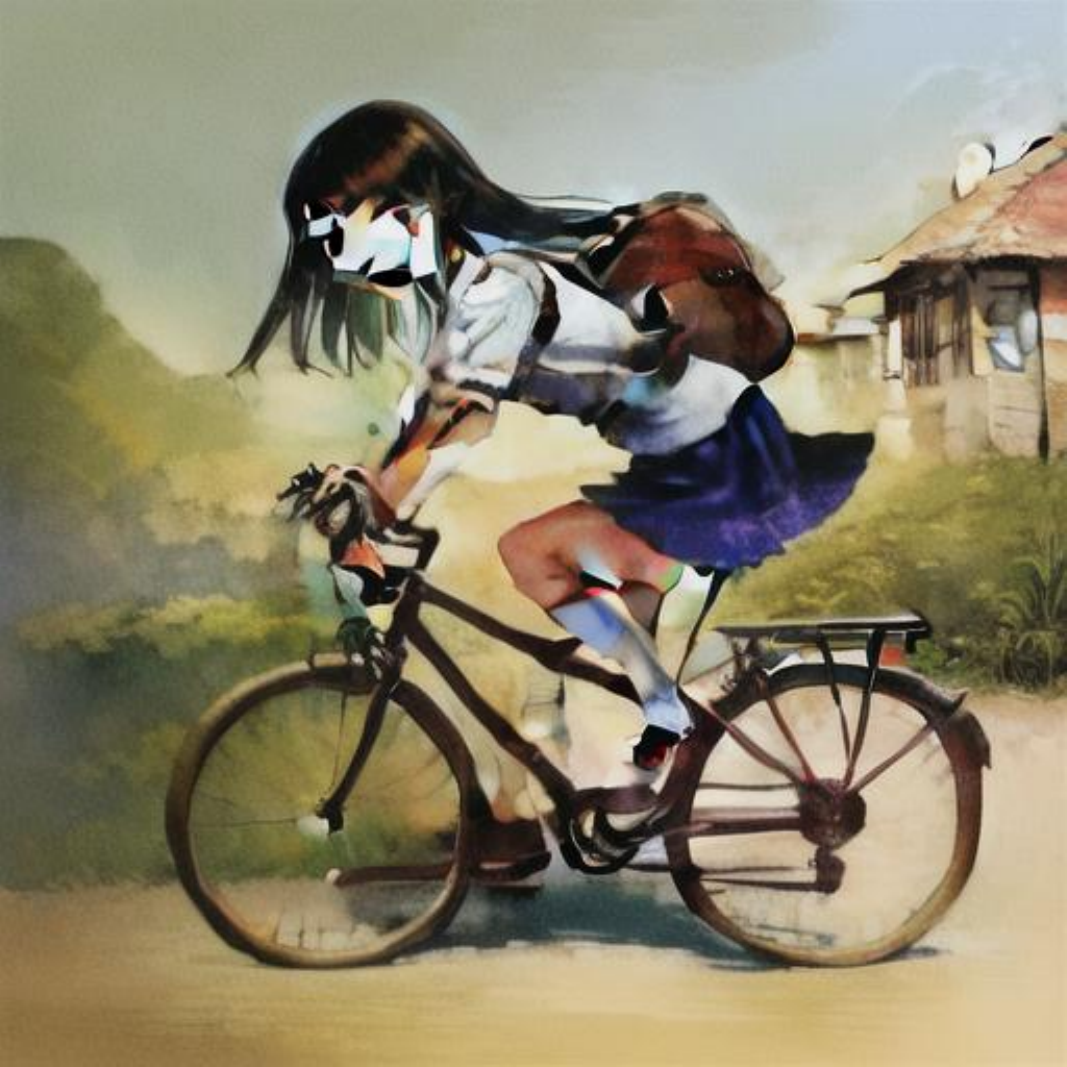}} & 
            \noindent\parbox[c]{0.17\columnwidth}{\includegraphics[width=0.17\columnwidth]{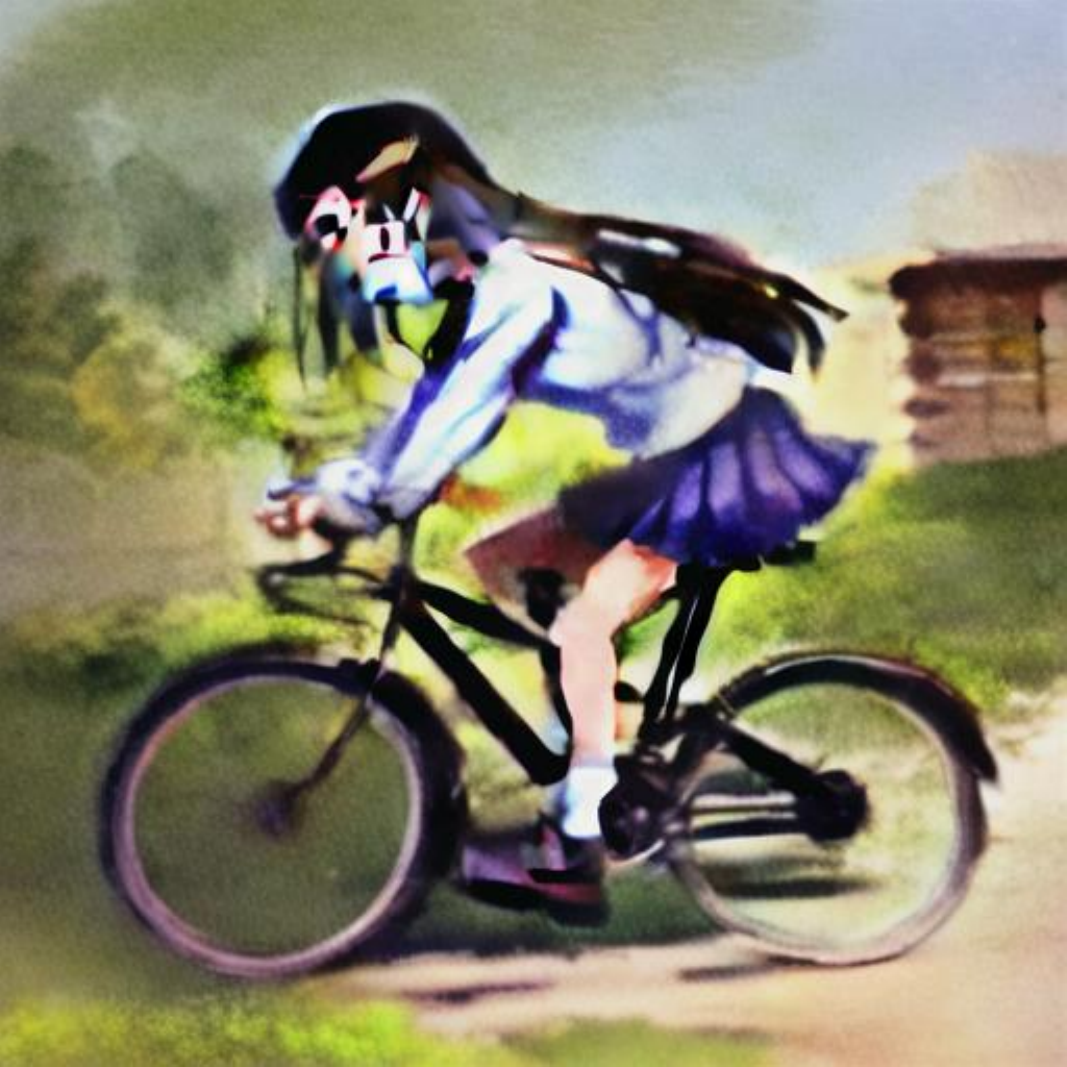}} & 
            \noindent\parbox[c]{0.17\columnwidth}{\includegraphics[width=0.17\columnwidth]{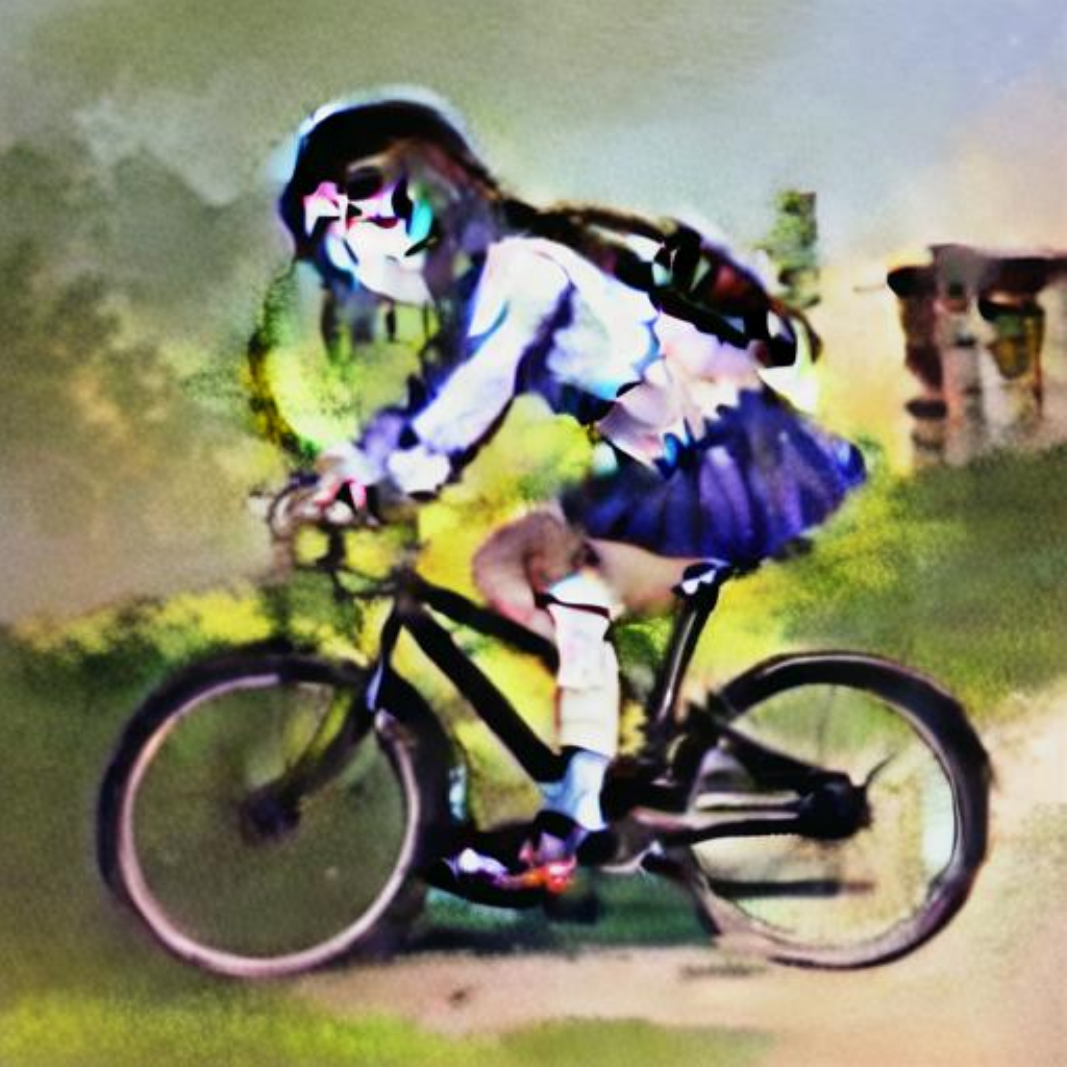}} \\
    
        \end{tabu}
    }

    \subcaptionbox{Prompt 2: bla bla bla}{
        \begin{tabu} to \textwidth {
            @{}
            l@{\hspace{6pt}}
            c@{\hspace{2pt}}
            c@{\hspace{2pt}}
            c@{\hspace{2pt}}
            c@{\hspace{2pt}}
            c@{}
        }
            % & \noindent\parbox[c]{0.17\columnwidth}{{DPM++ \cite{}}} 
            % & \multicolumn{4}{c}{\shortstack{\scriptsize DDIM \cite{} \\ \scriptsize 1000 steps}}
            & \multicolumn{1}{c}{\shortstack{\scriptsize $\beta = 0.2$}}
            & \multicolumn{1}{c}{\shortstack{\scriptsize $\beta = 0.4$}}
            & \multicolumn{1}{c}{\shortstack{\scriptsize $\beta = 0.6$}}
            & \multicolumn{1}{c}{\shortstack{\scriptsize $\beta = 0.8$}}
            & \multicolumn{1}{c}{\shortstack{\scriptsize $\beta = 0.9$}} \\
    
            \shortstack[l]{\scriptsize (a) w/ HB} &
            \noindent\parbox[c]{0.17\columnwidth}{\includegraphics[width=0.17\columnwidth]{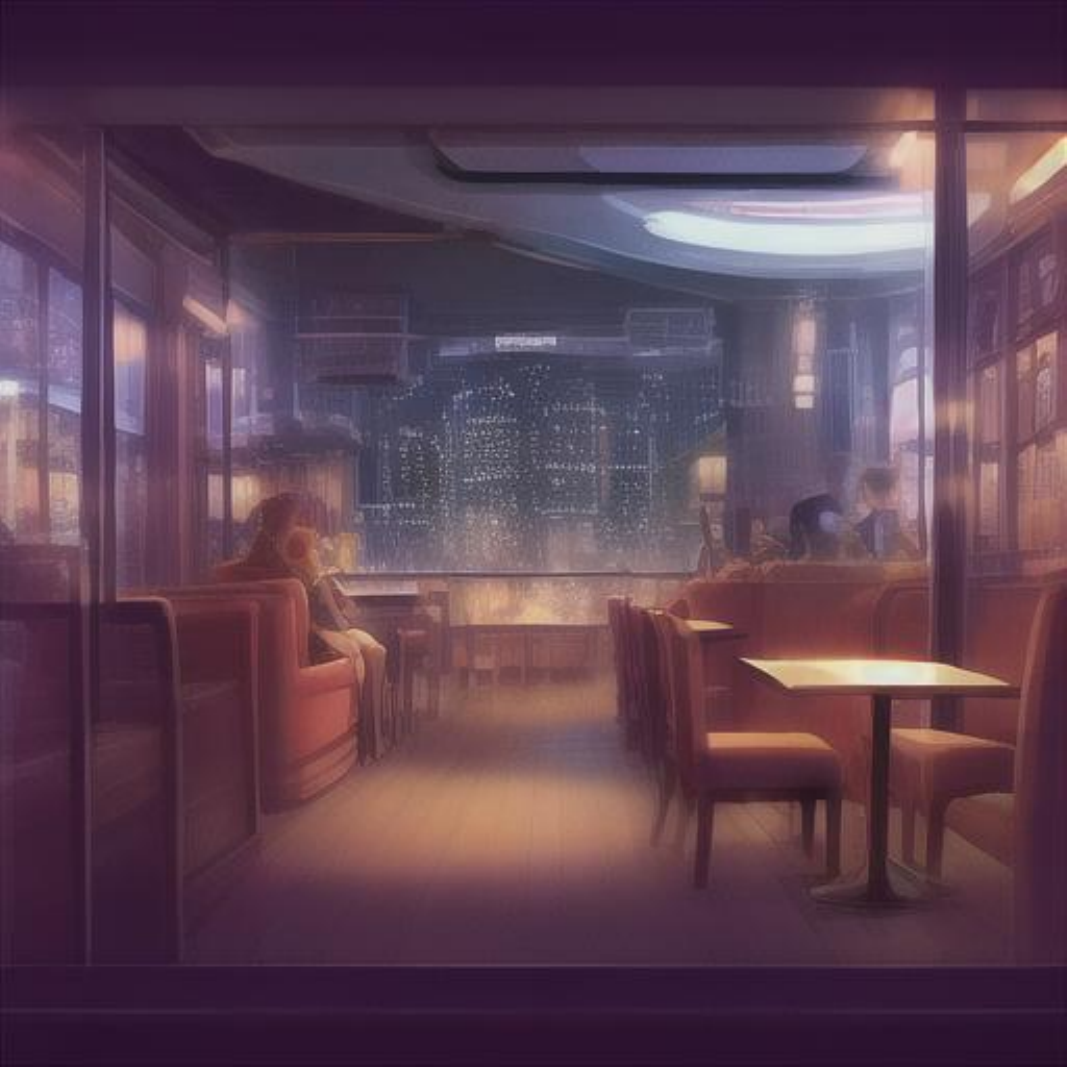}} & 
            \noindent\parbox[c]{0.17\columnwidth}{\includegraphics[width=0.17\columnwidth]{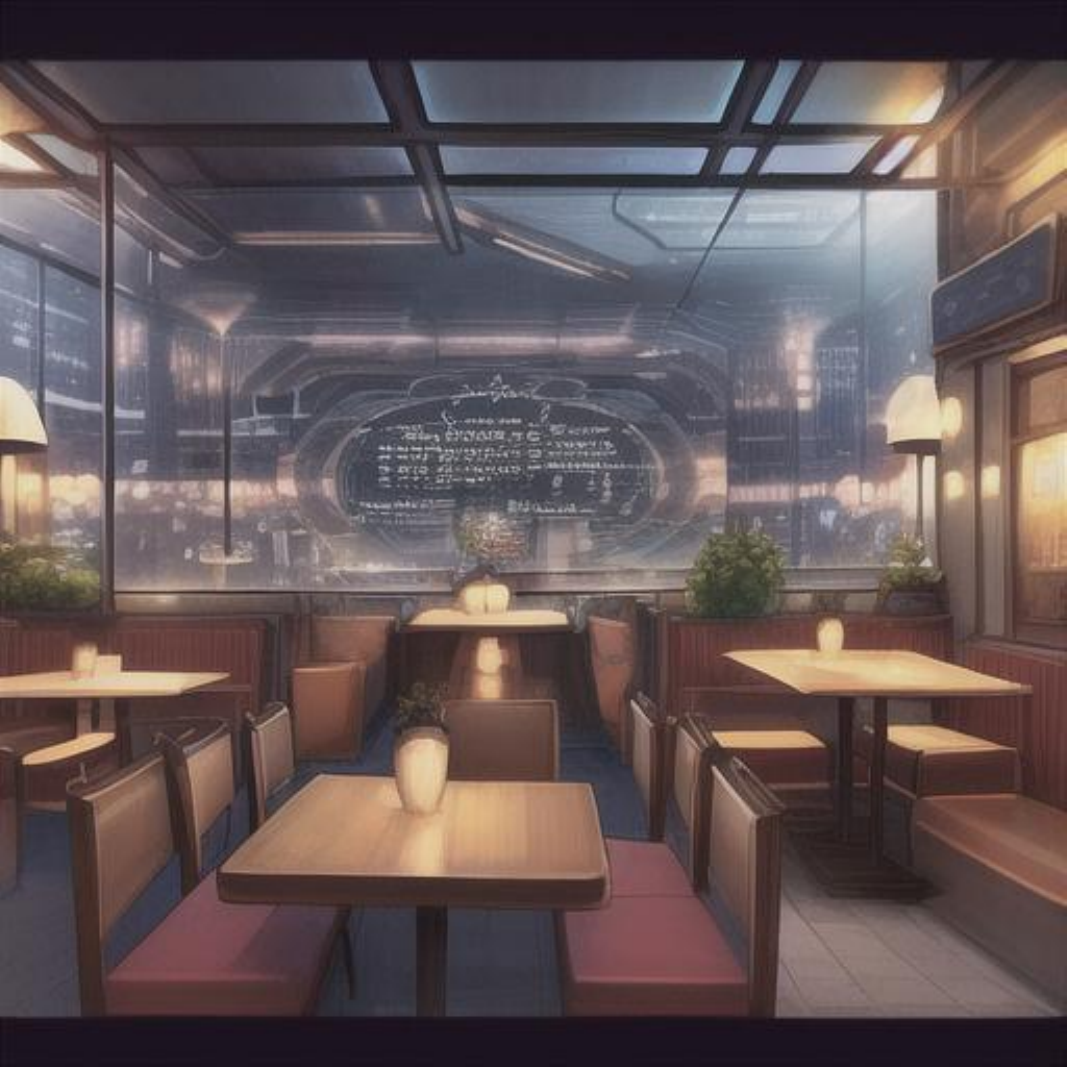}} & 
            \noindent\parbox[c]{0.17\columnwidth}{\includegraphics[width=0.17\columnwidth]{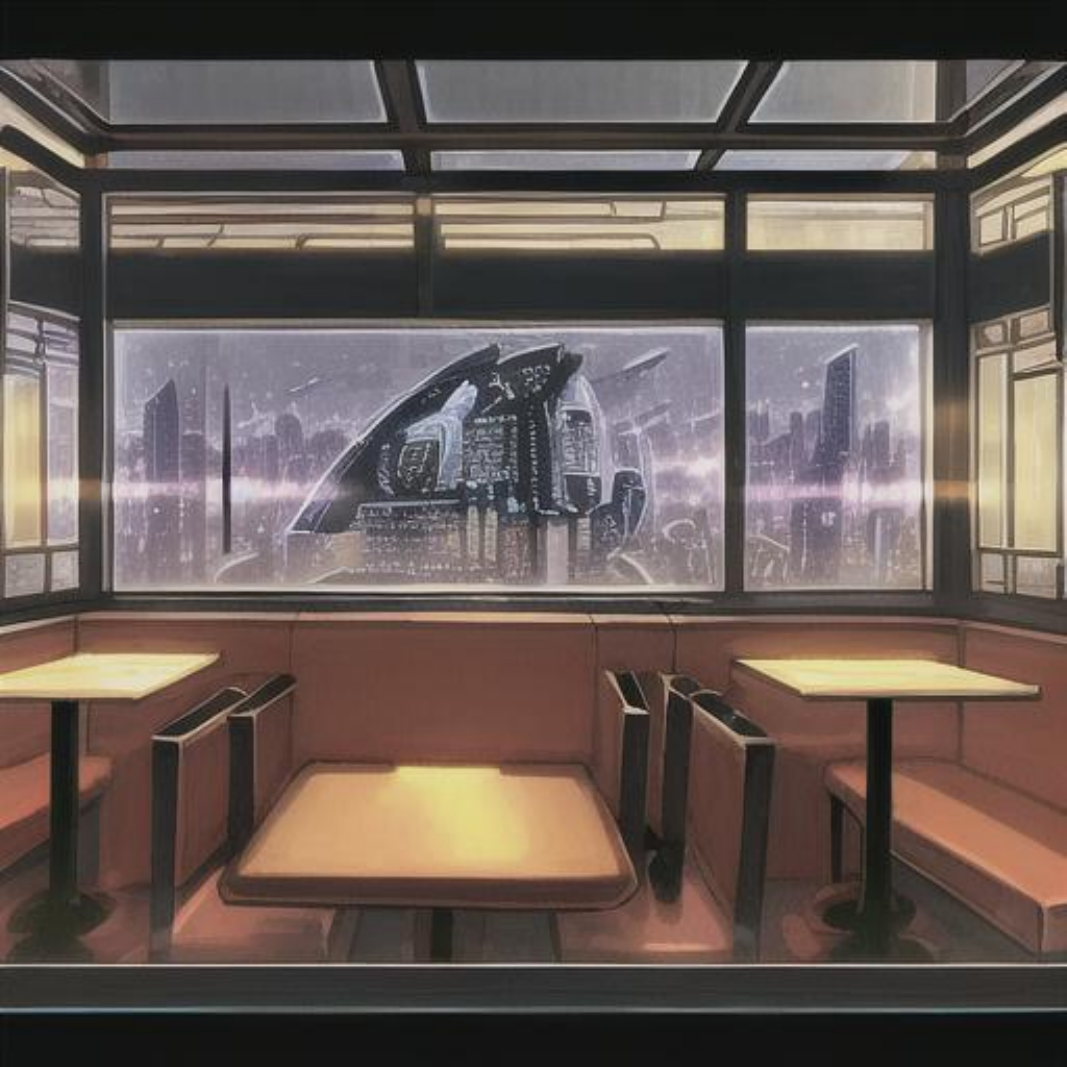}} & 
            \noindent\parbox[c]{0.17\columnwidth}{\includegraphics[width=0.17\columnwidth]{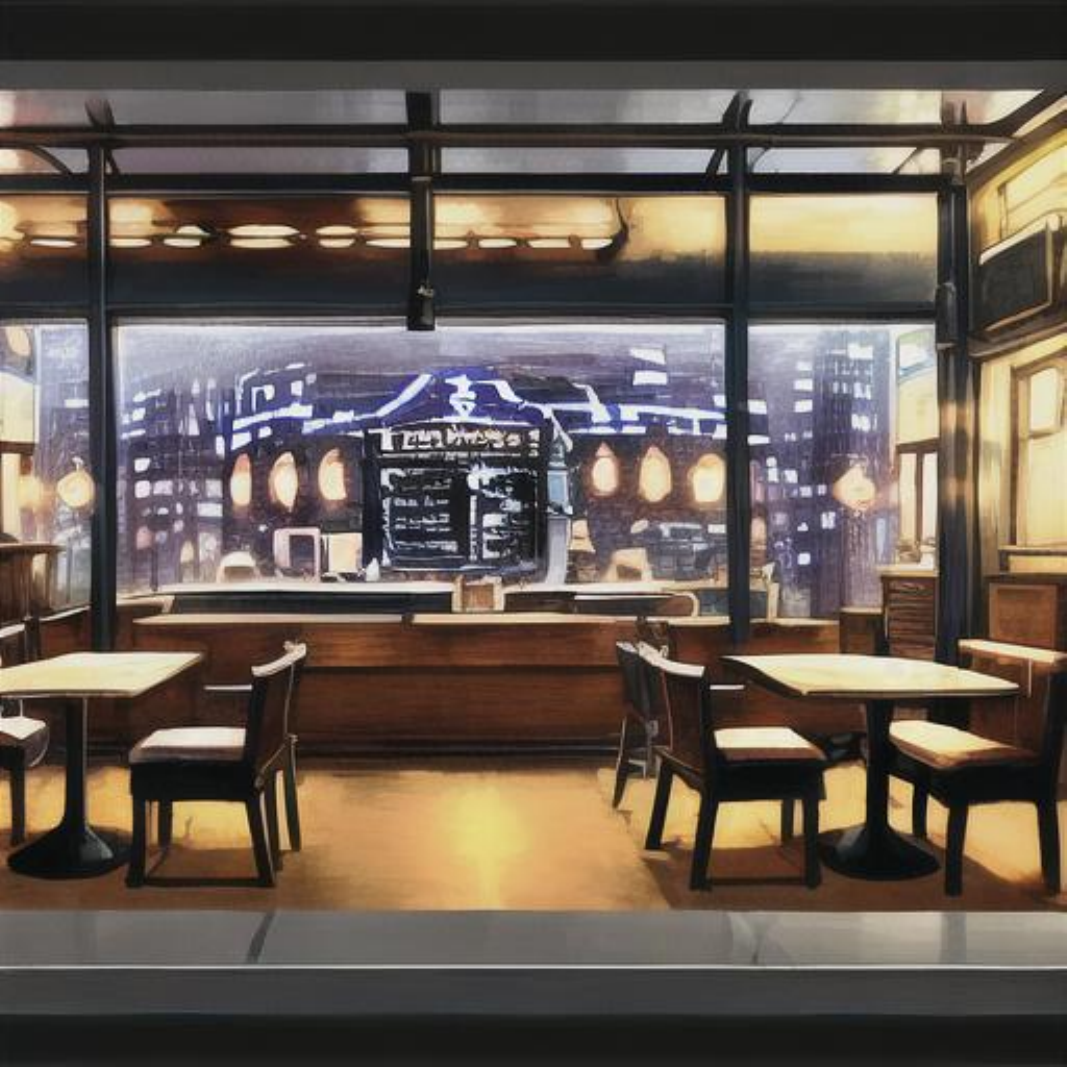}} & 
            \noindent\parbox[c]{0.17\columnwidth}{\includegraphics[width=0.17\columnwidth]{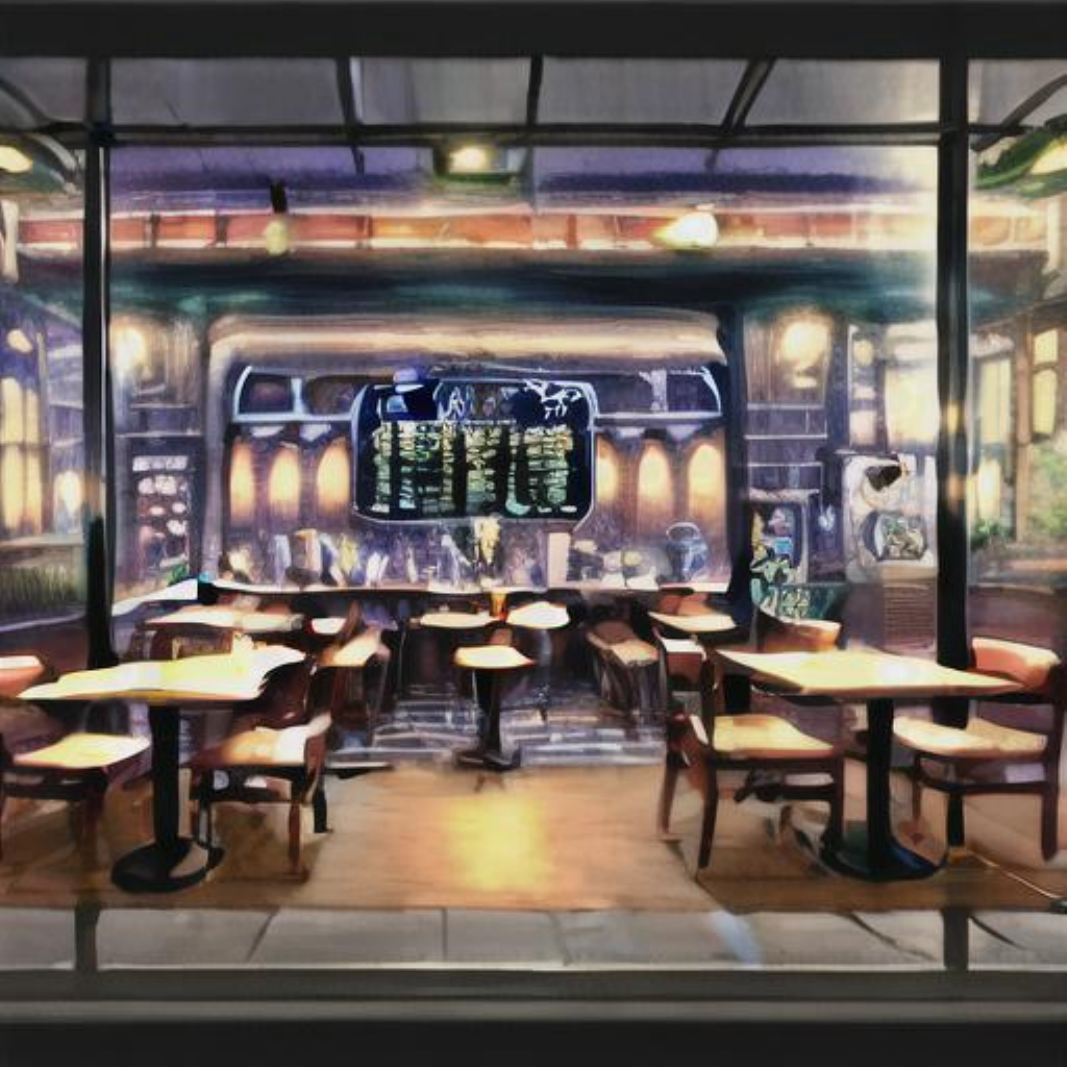}} \\
    
            & \multicolumn{1}{c}{\shortstack{\scriptsize $\beta = 0.2$}}
            & \multicolumn{1}{c}{\shortstack{\scriptsize $\beta = 0.4$}}
            & \multicolumn{1}{c}{\shortstack{\scriptsize $\beta = 0.6$}}
            & \multicolumn{1}{c}{\shortstack{\scriptsize $\beta = 0.8$}}
            & \multicolumn{1}{c}{\shortstack{\scriptsize $\beta = 0.9$}} \\
    
            \shortstack[l]{\scriptsize (a) w/ NT} &
            \noindent\parbox[c]{0.17\columnwidth}{\includegraphics[width=0.17\columnwidth]{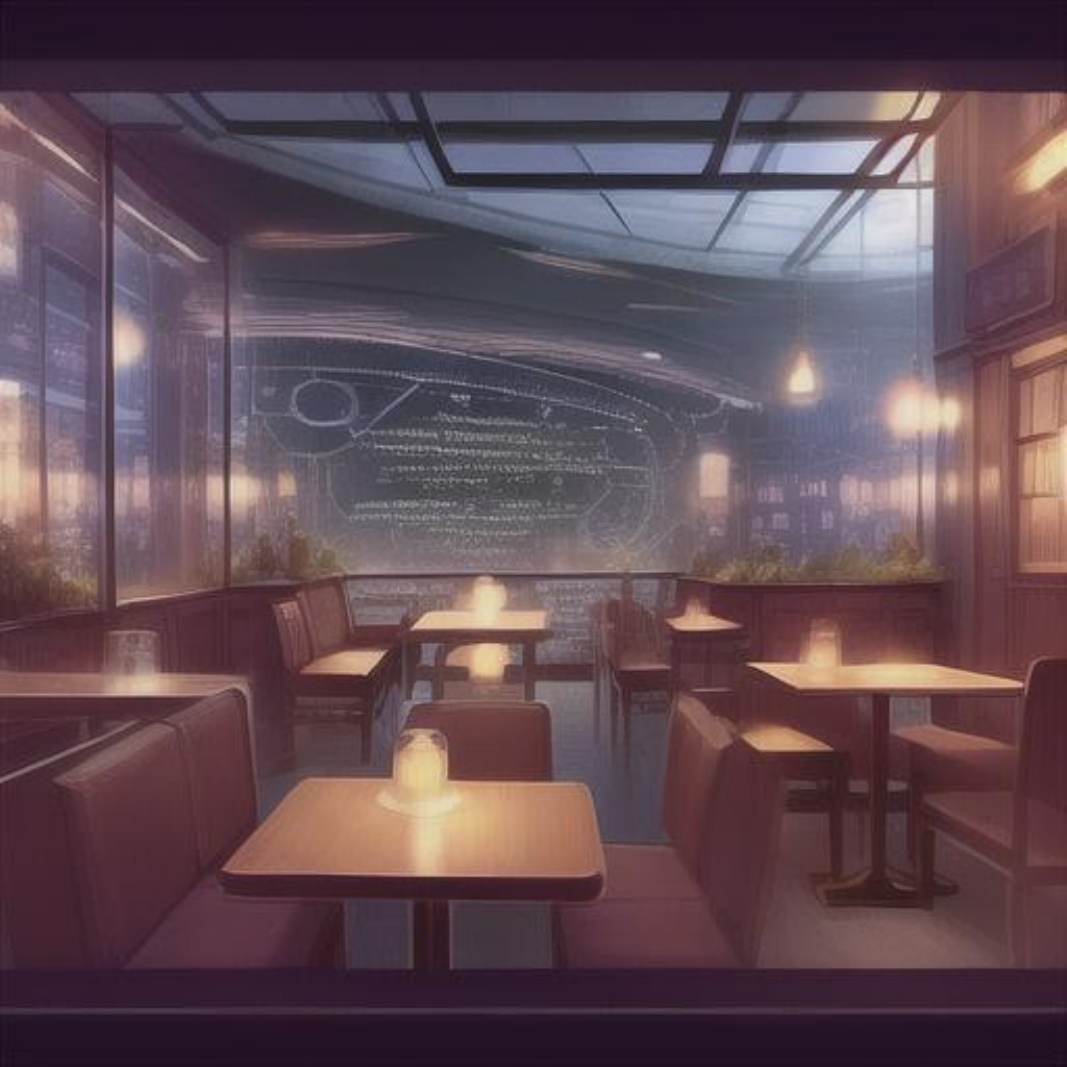}} & 
            \noindent\parbox[c]{0.17\columnwidth}{\includegraphics[width=0.17\columnwidth]{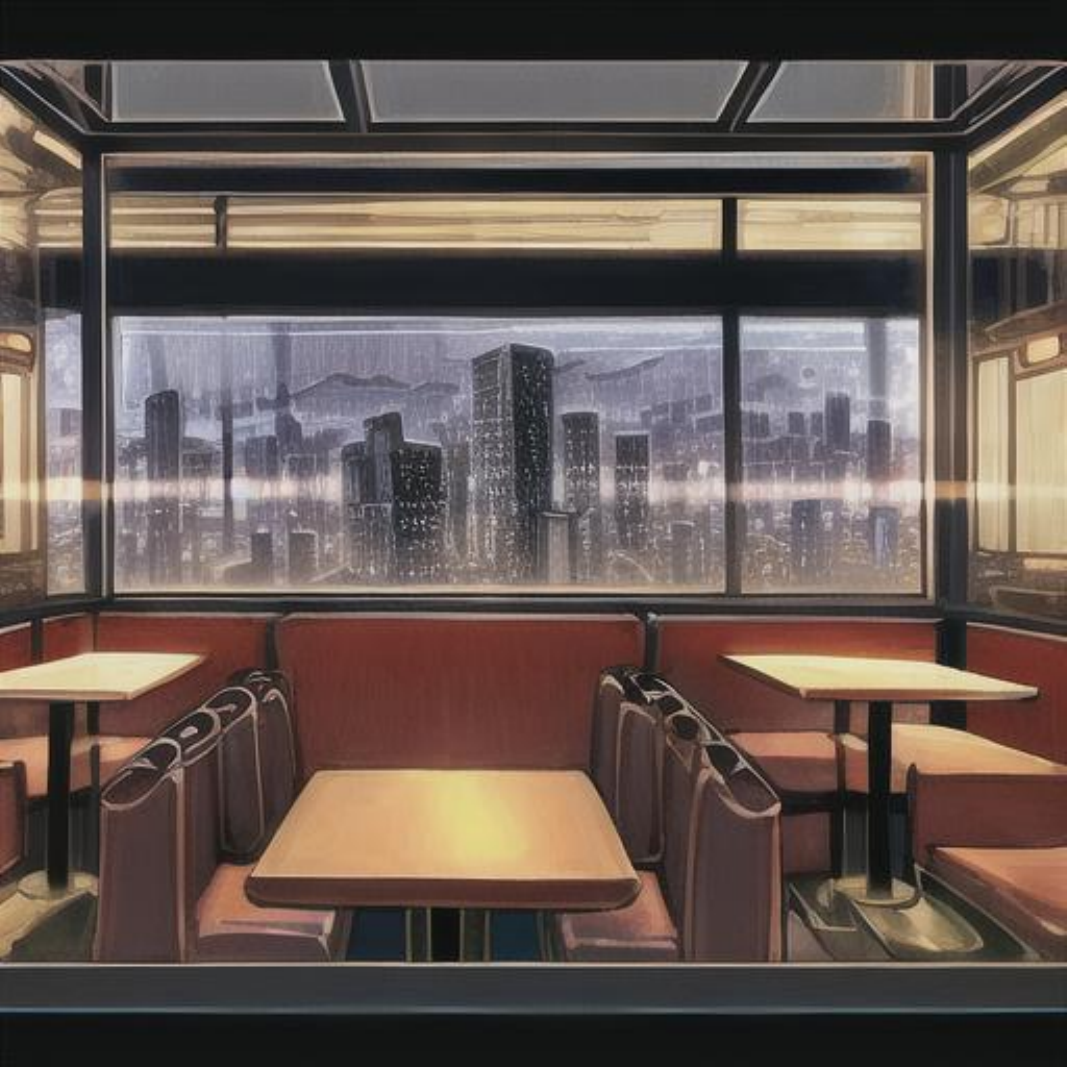}} & 
            \noindent\parbox[c]{0.17\columnwidth}{\includegraphics[width=0.17\columnwidth]{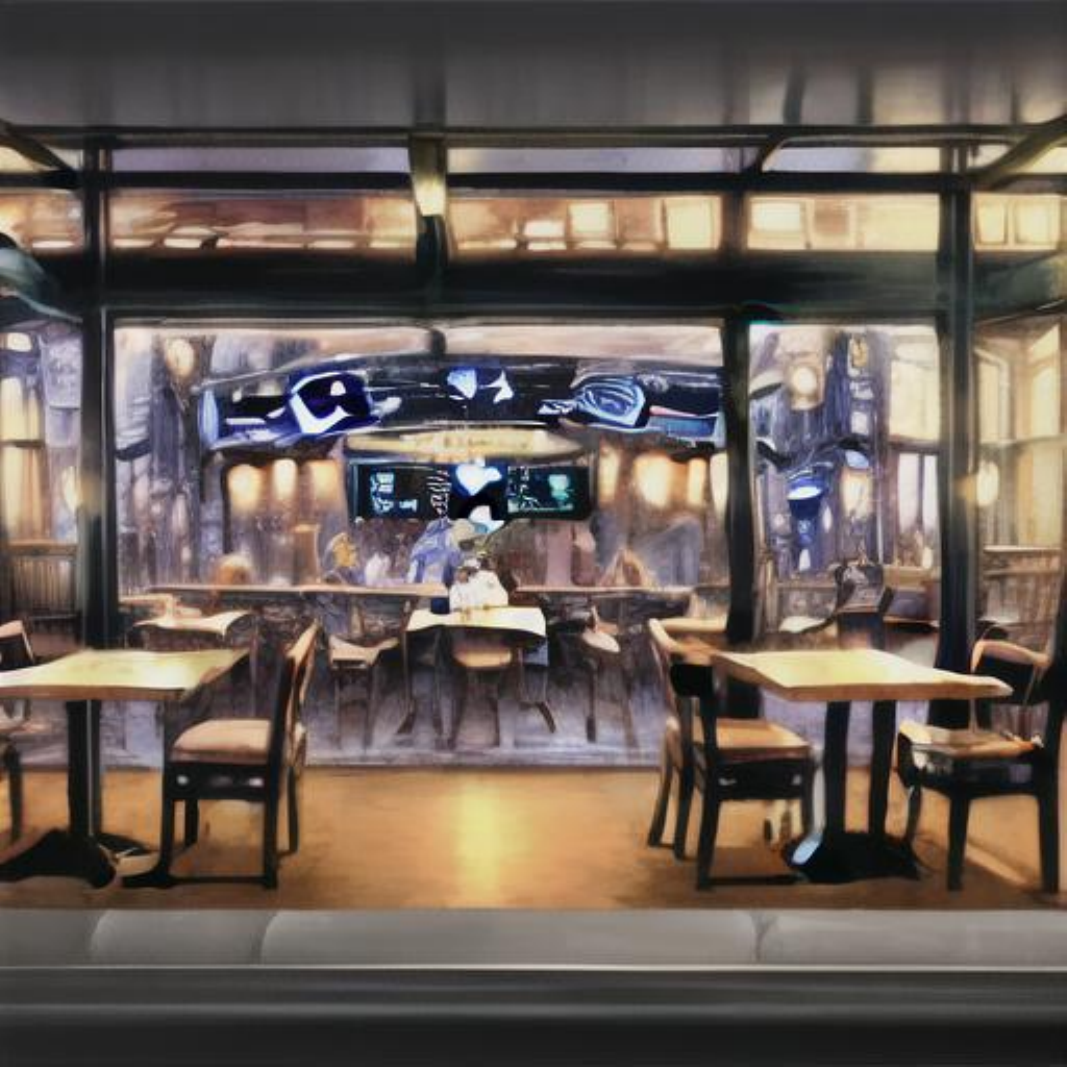}} & 
            \noindent\parbox[c]{0.17\columnwidth}{\includegraphics[width=0.17\columnwidth]{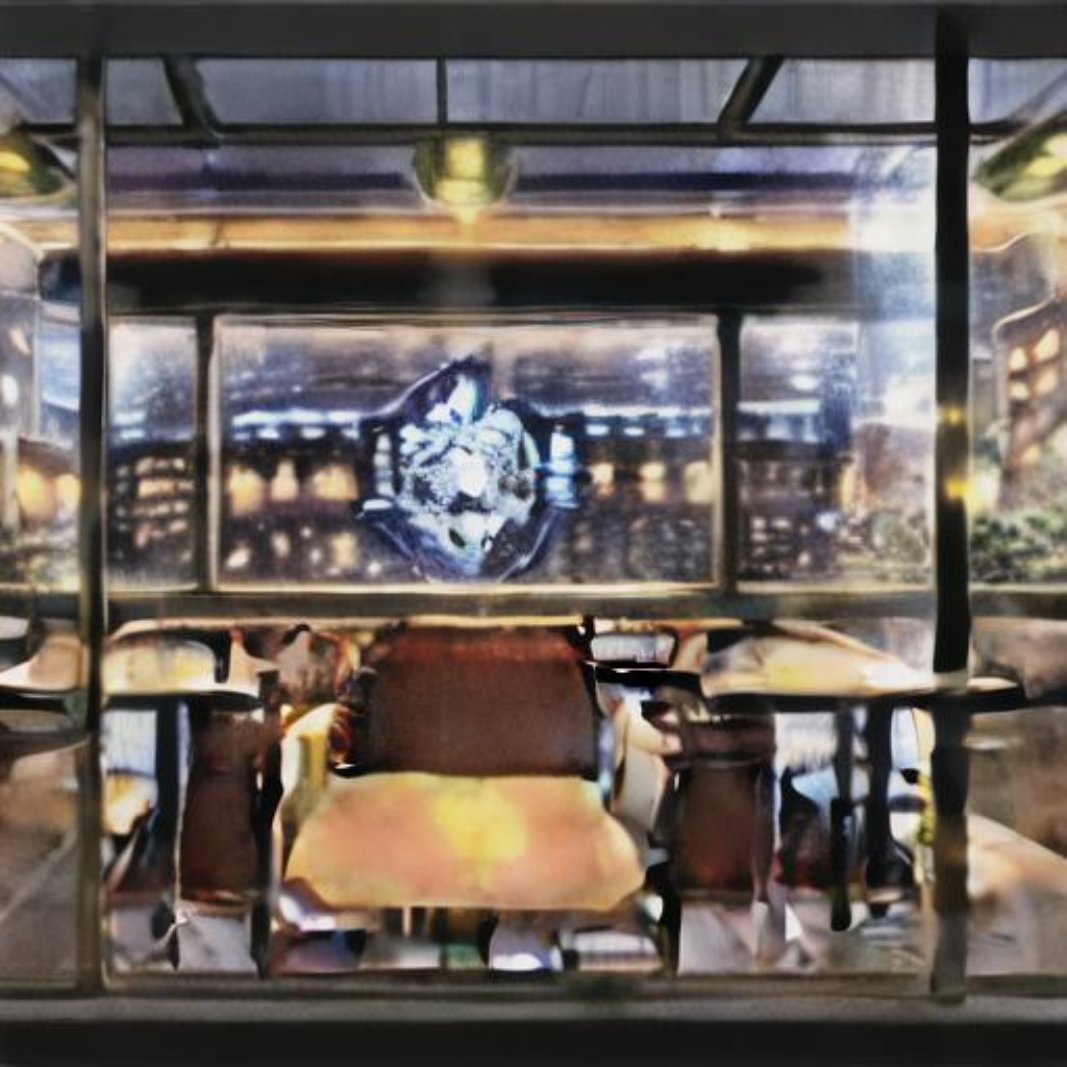}} & 
            \noindent\parbox[c]{0.17\columnwidth}{\includegraphics[width=0.17\columnwidth]{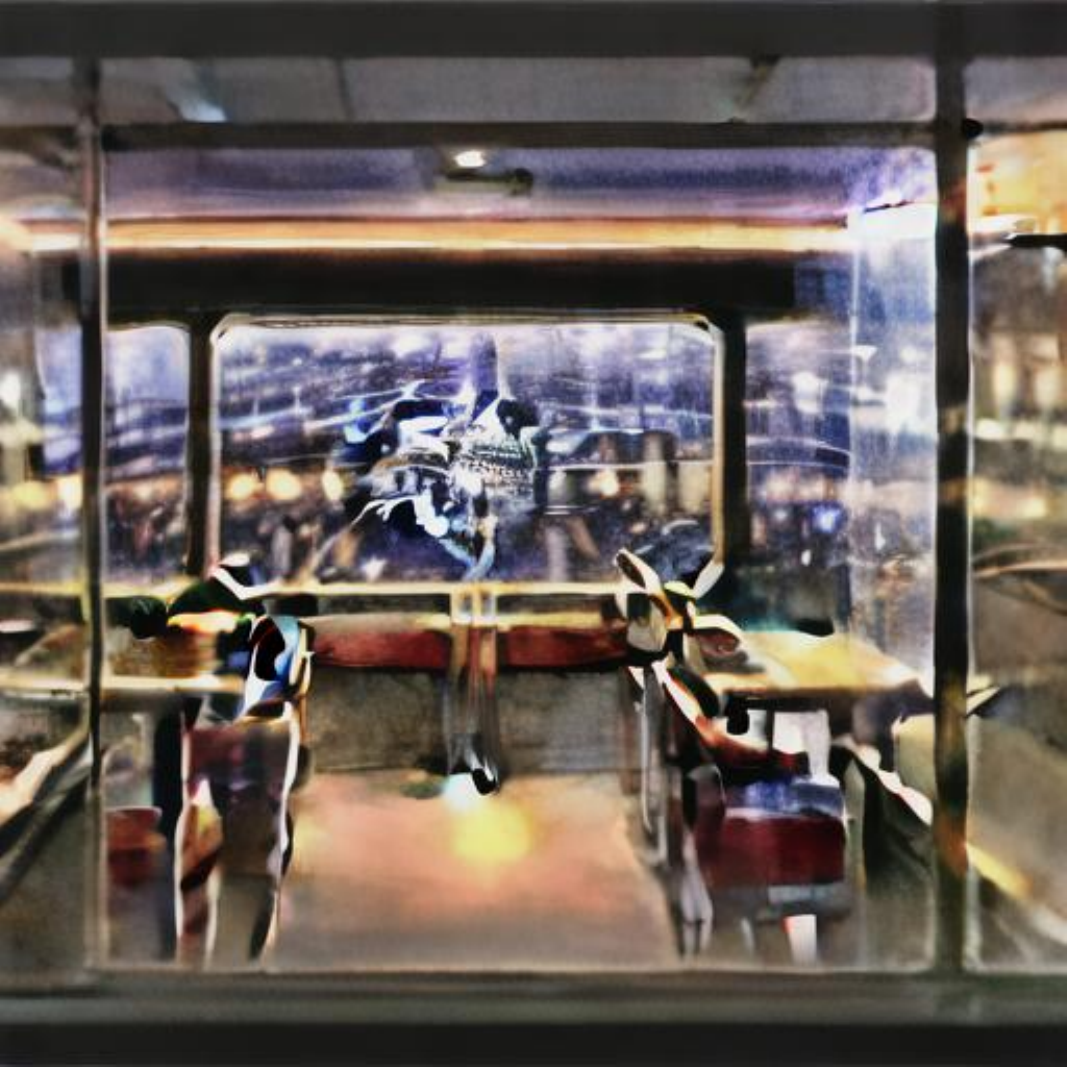}} \\
    
        \end{tabu}
    }

    \subcaptionbox{Prompt 3: bla bla bla}{
        \begin{tabu} to \textwidth {
            @{}
            l@{\hspace{6pt}}
            c@{\hspace{2pt}}
            c@{\hspace{2pt}}
            c@{\hspace{2pt}}
            c@{\hspace{2pt}}
            c@{}
        }
            % & \noindent\parbox[c]{0.17\columnwidth}{{DPM++ \cite{}}} 
            % & \multicolumn{4}{c}{\shortstack{\scriptsize DDIM \cite{} \\ \scriptsize 1000 steps}}
            & \multicolumn{1}{c}{\shortstack{\scriptsize $\beta = 0.2$}}
            & \multicolumn{1}{c}{\shortstack{\scriptsize $\beta = 0.4$}}
            & \multicolumn{1}{c}{\shortstack{\scriptsize $\beta = 0.6$}}
            & \multicolumn{1}{c}{\shortstack{\scriptsize $\beta = 0.8$}}
            & \multicolumn{1}{c}{\shortstack{\scriptsize $\beta = 0.9$}} \\
    
            \shortstack[l]{\scriptsize (a) w/ HB} &
            \noindent\parbox[c]{0.17\columnwidth}{\includegraphics[width=0.17\columnwidth]{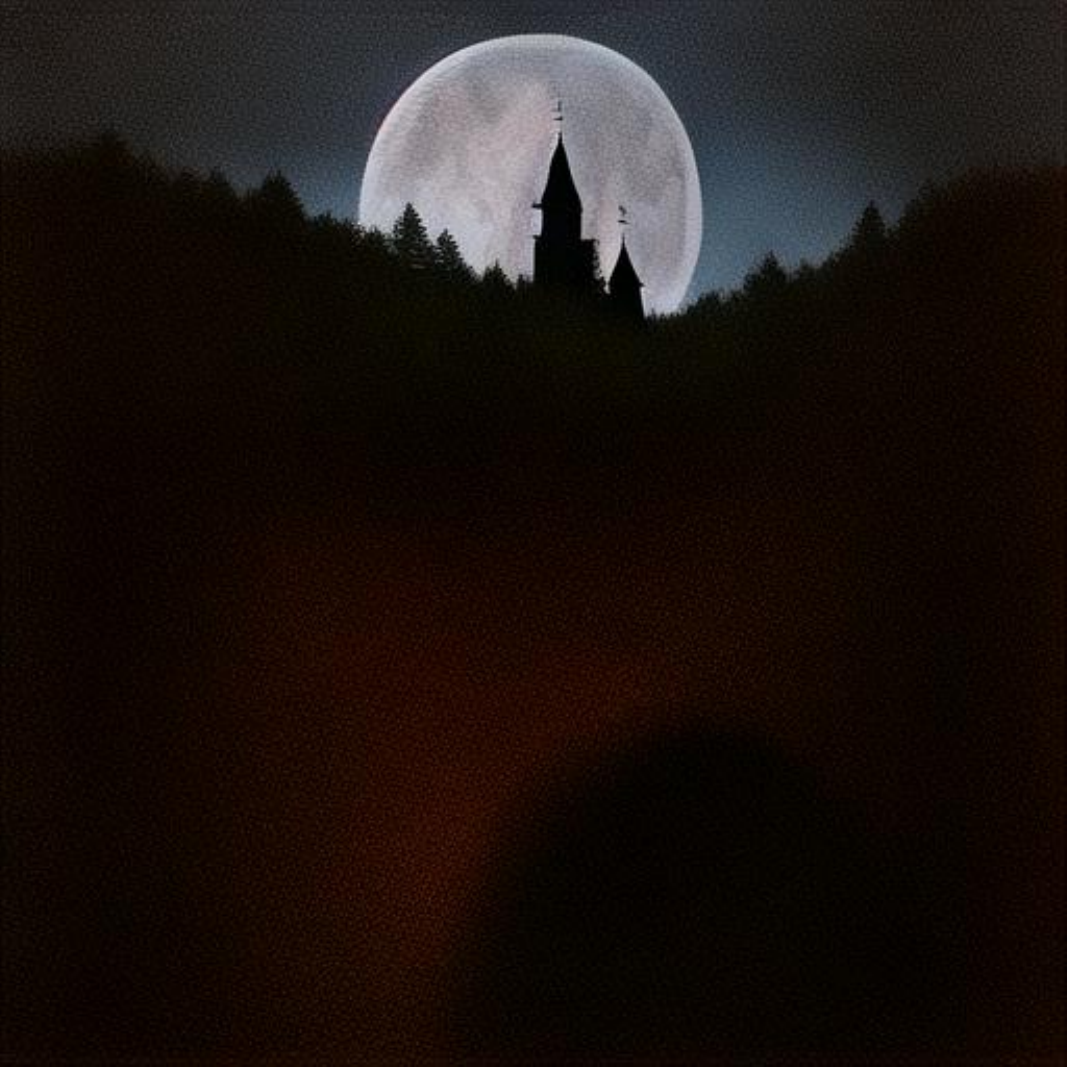}} & 
            \noindent\parbox[c]{0.17\columnwidth}{\includegraphics[width=0.17\columnwidth]{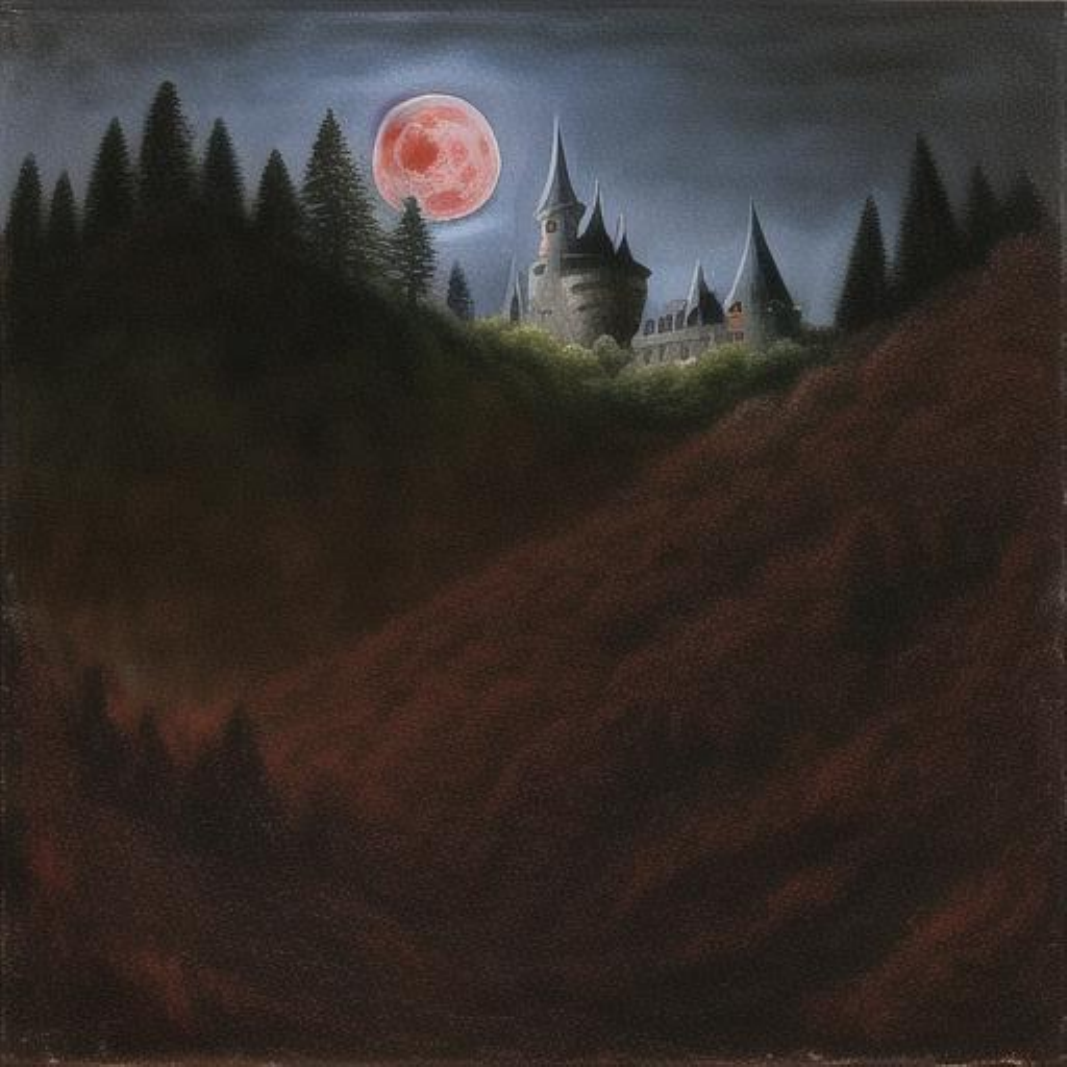}} & 
            \noindent\parbox[c]{0.17\columnwidth}{\includegraphics[width=0.17\columnwidth]{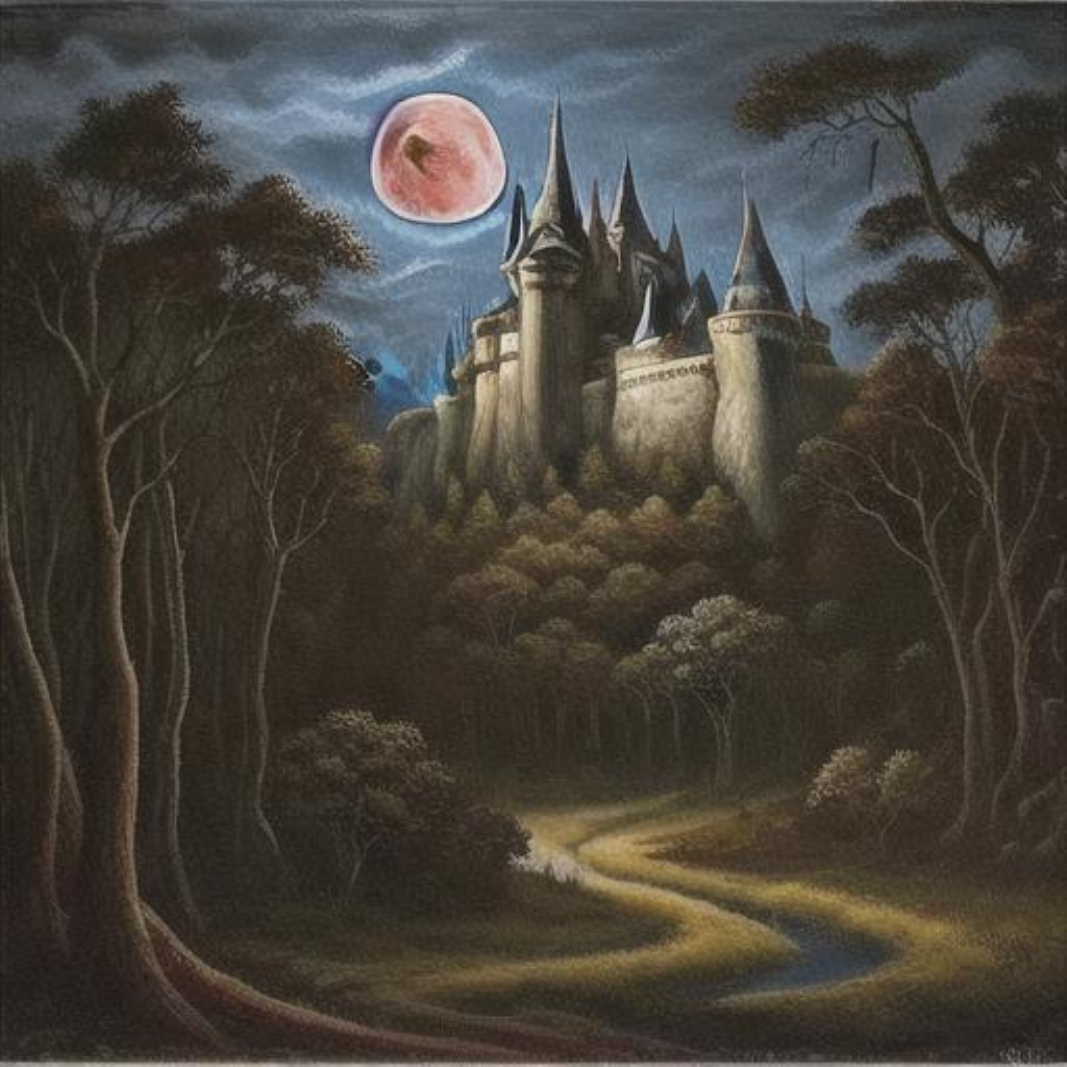}} & 
            \noindent\parbox[c]{0.17\columnwidth}{\includegraphics[width=0.17\columnwidth]{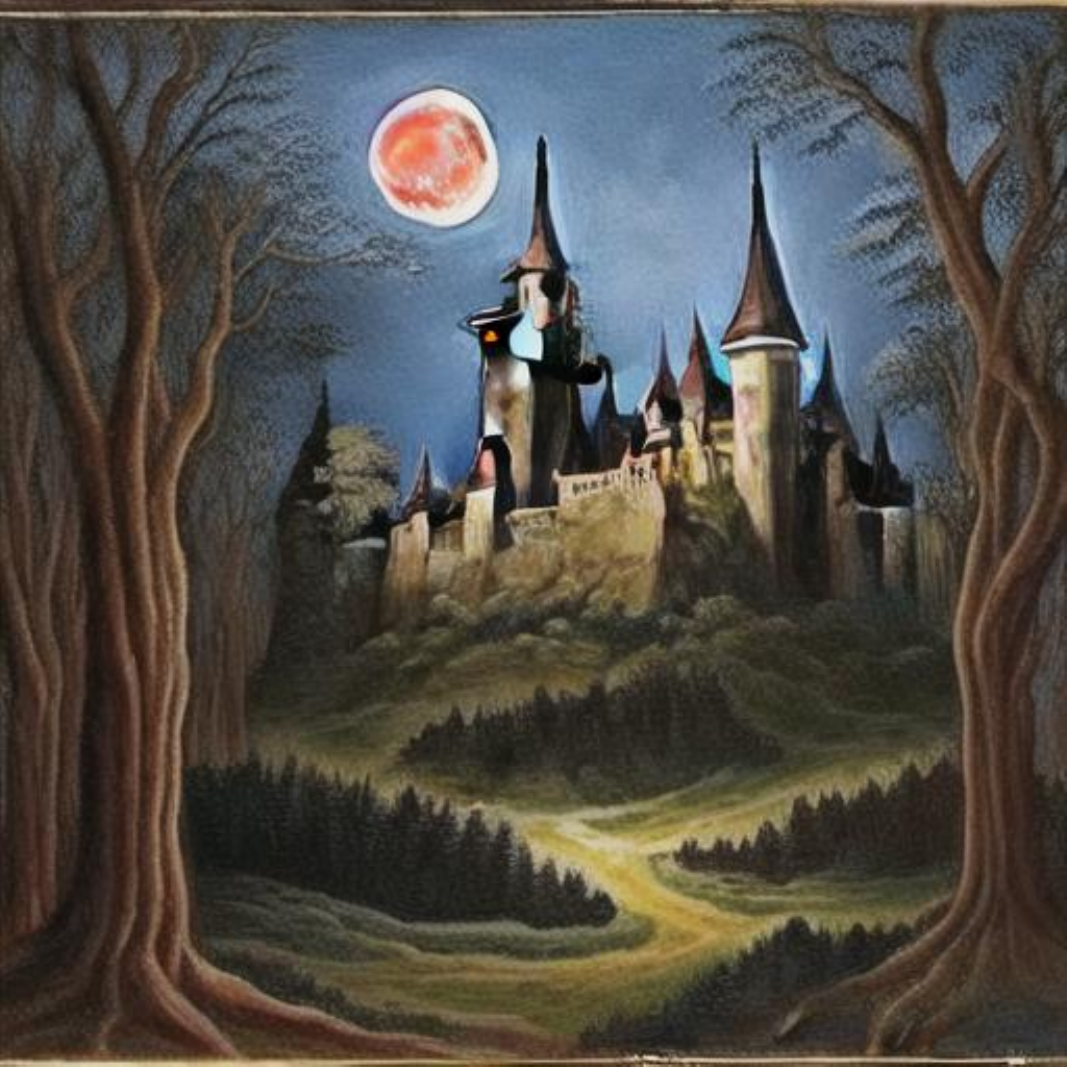}} & 
            \noindent\parbox[c]{0.17\columnwidth}{\includegraphics[width=0.17\columnwidth]{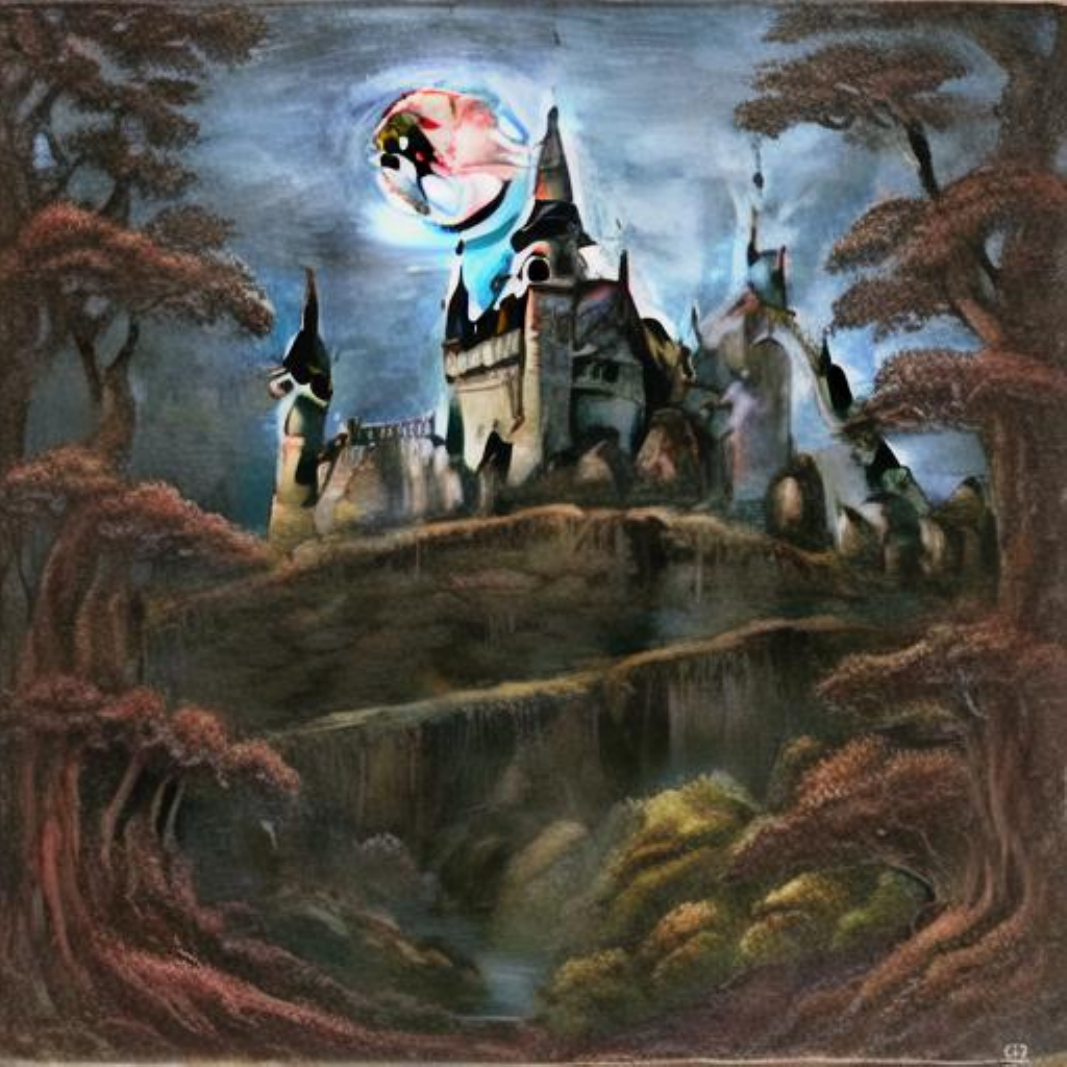}} \\
    
            & \multicolumn{1}{c}{\shortstack{\scriptsize $\beta = 0.2$}}
            & \multicolumn{1}{c}{\shortstack{\scriptsize $\beta = 0.4$}}
            & \multicolumn{1}{c}{\shortstack{\scriptsize $\beta = 0.6$}}
            & \multicolumn{1}{c}{\shortstack{\scriptsize $\beta = 0.8$}}
            & \multicolumn{1}{c}{\shortstack{\scriptsize $\beta = 0.9$}} \\
    
            \shortstack[l]{\scriptsize (a) w/ NT} &
            \noindent\parbox[c]{0.17\columnwidth}{\includegraphics[width=0.17\columnwidth]{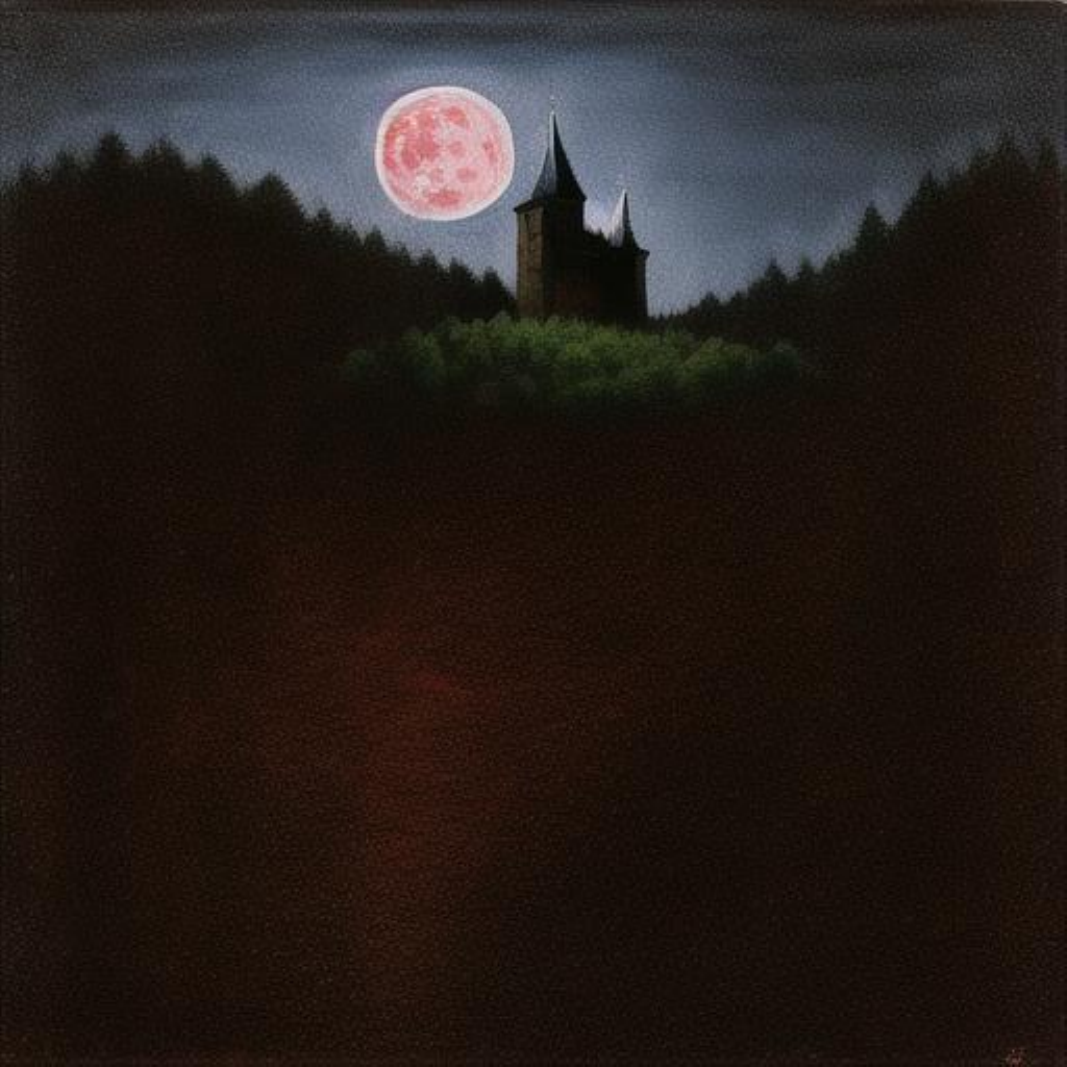}} & 
            \noindent\parbox[c]{0.17\columnwidth}{\includegraphics[width=0.17\columnwidth]{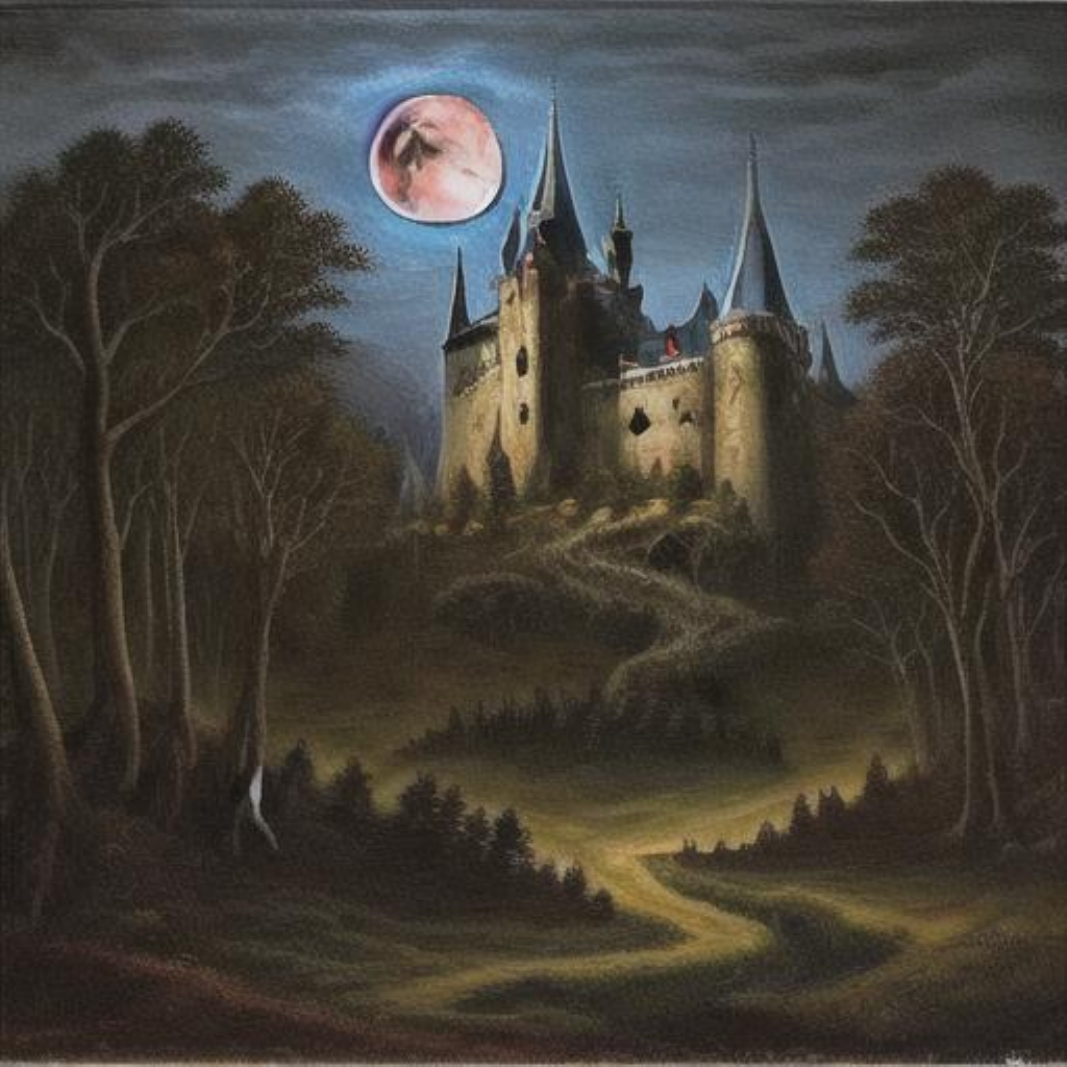}} & 
            \noindent\parbox[c]{0.17\columnwidth}{\includegraphics[width=0.17\columnwidth]{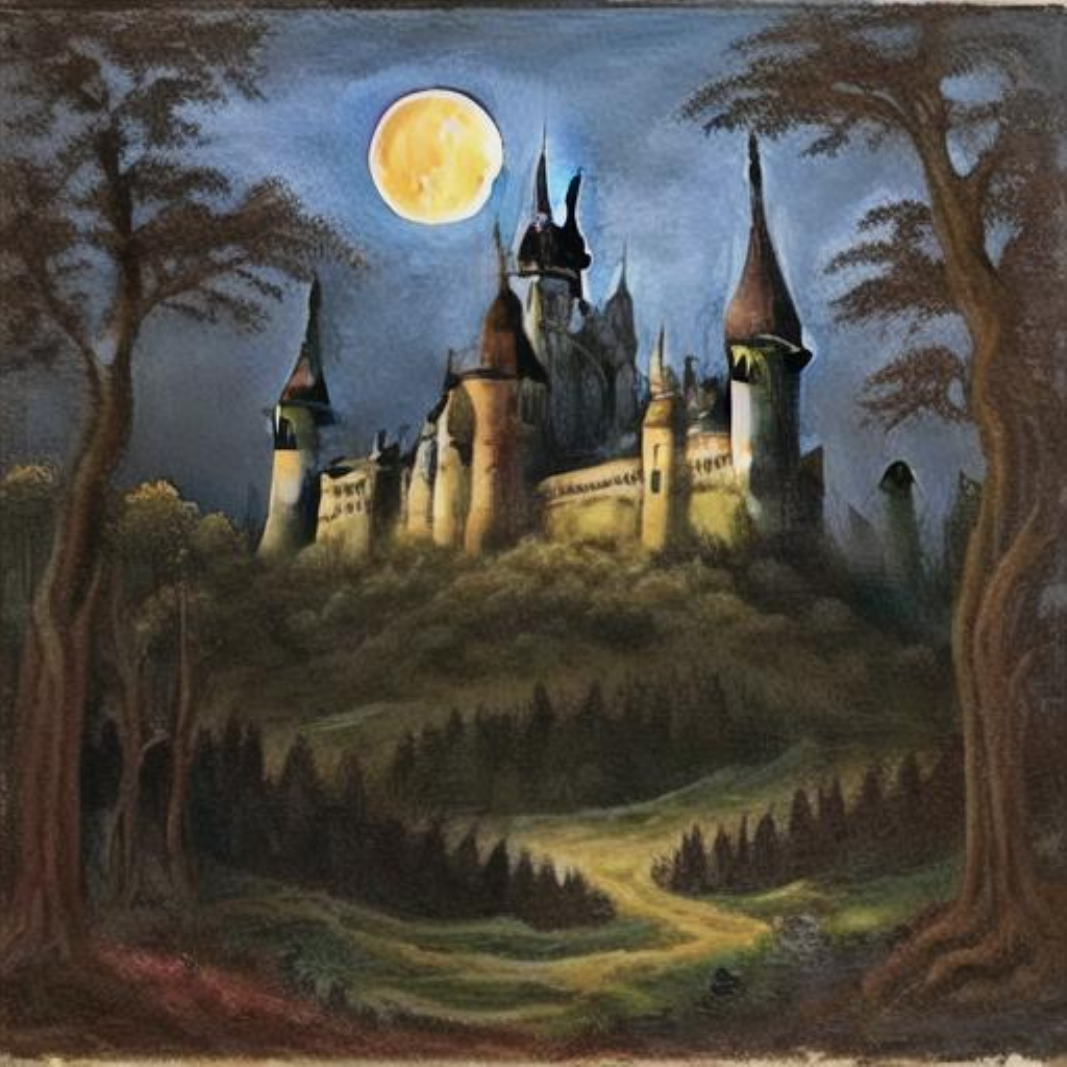}} & 
            \noindent\parbox[c]{0.17\columnwidth}{\includegraphics[width=0.17\columnwidth]{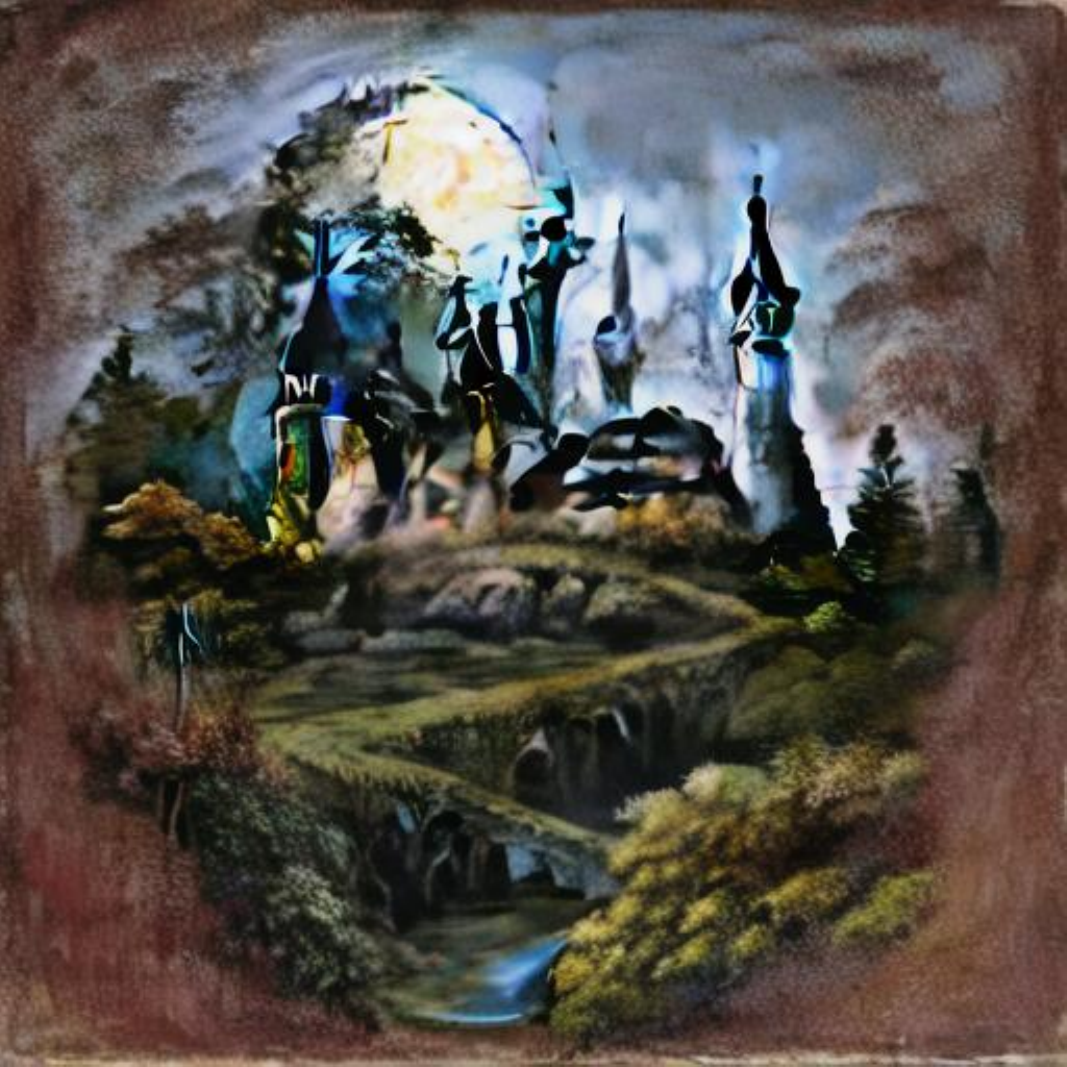}} & 
            \noindent\parbox[c]{0.17\columnwidth}{\includegraphics[width=0.17\columnwidth]{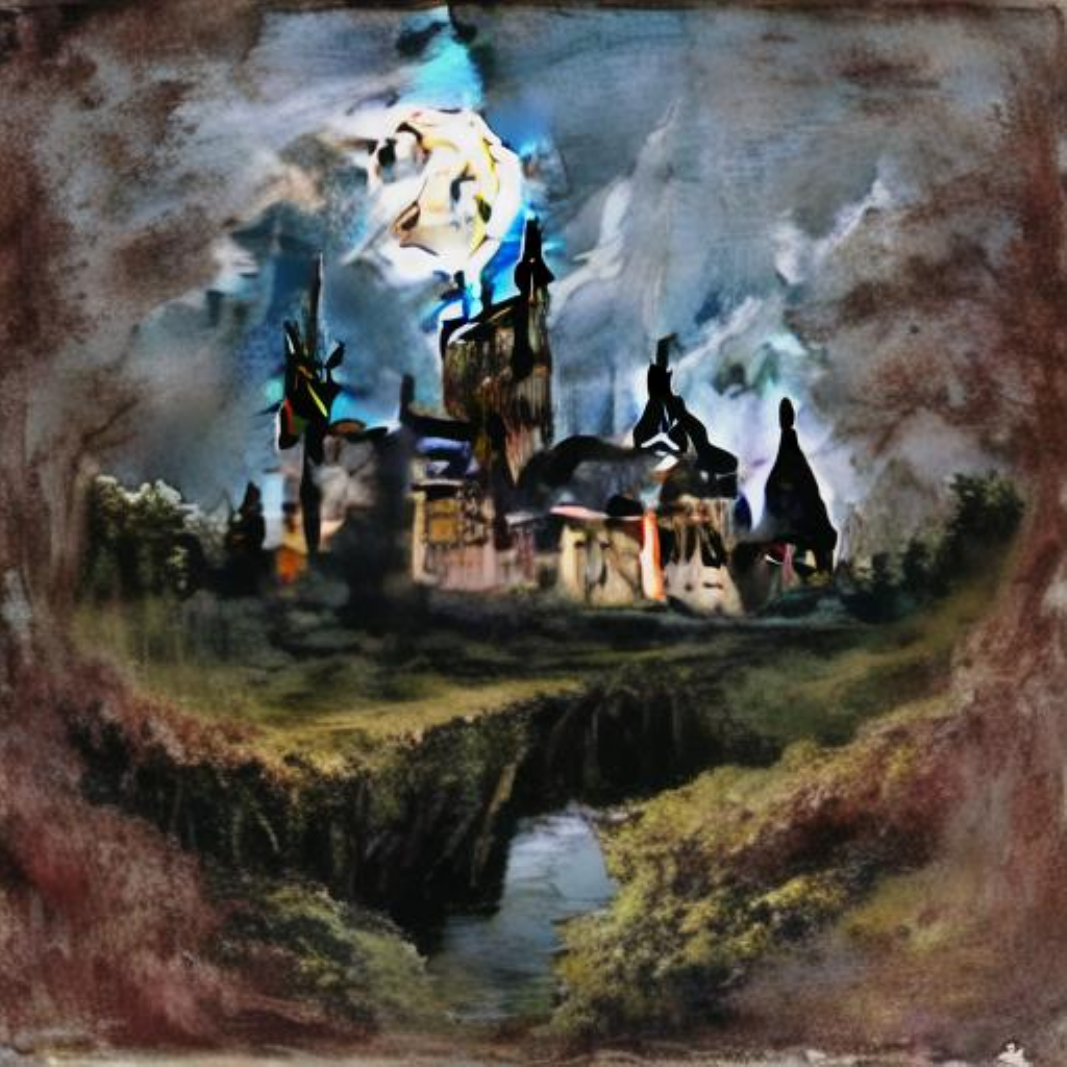}} \\
    
        \end{tabu}
    }
    \caption{Comparison between HB and Nesterov momentum on PLMS4}
\end{figure}
